# Supplementary material for: Parametric bootstrap inference for stratified models with high-dimensional nuisance specifications
Source: arXiv:2010.16186 source file (2022-01-06)
Supplement: Supplementary file 1 [file boot-strata-supplementary-submission0.pdf]

# Supplementary Material for Parametric bootstrap inference for stratified models with high-dimensional nuisance specifications

Ruggero Bellio<sup>\*1</sup>, Ioannis Kosmidis<sup>†2, 3</sup>, Nicola Sartori<sup>‡4</sup>, and Alessandra Salvan<sup>§4</sup>

<sup>1</sup>Department of Economics and Statistics, University of Udine, Udine, 33100, Italy

<sup>2</sup>Department of Statistics, University of Warwick, Coventry, CV4 7AL, UK

<sup>3</sup>The Alan Turing Institute, London, NW1 2DB, UK

<sup>4</sup>Department of Statistical Sciences, University of Padova, 35121, Padova, Italy

October 30, 2020

## Full set of simulation results

In this document, we report the full set of results of the simulation studies described in the main paper. For each model, simulation results for the 23 statistics are visualized. For plotting purposes, the statistics have been split in two groups. Table [S1](#) lists the first group, and Table [S2](#) the second one.

---

<sup>\*</sup>ruggero.bellio@uniud.it

<sup>†</sup>ioannis.kosmidis@warwick.ac.uk

<sup>‡</sup>sartori@stat.unipd.it

<sup>§</sup>salvan@stat.unipd.it

Table S1: Statistics computed in the simulation experiments (first group for plotting).

| Statistic                        | Plotting Symbol | Description                                                          |
|----------------------------------|-----------------|----------------------------------------------------------------------|
| $R(\psi)$                        | $R$             | Signed likelihood root                                               |
| $S(\psi)$                        | $S$             | Score statistic                                                      |
| $T(\psi)$                        | $T$             | Wald statistic                                                       |
| $\Phi^{-1}\{\hat{p}_1^T(\psi)\}$ | $T^u$           | Transformed $p$ -value from unconstrained bootstrap of $T(\psi)$     |
| $\Phi^{-1}\{\hat{p}_2^T(\psi)\}$ | $T^c$           | Transformed $p$ -value from constrained bootstrap of $T(\psi)$       |
| $\Phi^{-1}\{\hat{p}_1^S(\psi)\}$ | $S^u$           | Transformed $p$ -value from unconstrained bootstrap of $S(\psi)$     |
| $\Phi^{-1}\{\hat{p}_2^S(\psi)\}$ | $S^c$           | Transformed $p$ -value from constrained bootstrap of $S(\psi)$       |
| $\Phi^{-1}\{\hat{p}_1^R(\psi)\}$ | $R^u$           | Transformed $p$ -value from unconstrained bootstrap of $R(\psi)$     |
| $\Phi^{-1}\{\hat{p}_2^R(\psi)\}$ | $R^c$           | Transformed $p$ -value from constrained bootstrap of $R(\psi)$       |
| $R^*(\psi)$                      | $R^*$           | Modified signed likelihood root                                      |
| $R_m(\psi)$                      | $R_m$           | Signed likelihood root computed from the modified profile likelihood |

Table S2: Statistics computed in the simulation experiments (second group for plotting). The mean  $\hat{\mu}^R$  and the standard deviation  $\hat{\sigma}^R$  of  $R(\psi)$  are estimated through unconstrained bootstrap, by simulating from the model at  $\theta = \hat{\theta}$ , and likewise for  $S(\psi)$  and  $T(\psi)$ . The mean  $\tilde{\mu}^R$  and the standard deviation  $\tilde{\sigma}^R$  of  $R(\psi)$  are estimated through constrained bootstrap, by simulating from the model at  $\theta = \hat{\theta}_\psi$ , and likewise for  $S(\psi)$  and  $T(\psi)$ .

| Statistic                                    | Plotting Symbol | Description                                                     |
|----------------------------------------------|-----------------|-----------------------------------------------------------------|
| $T(\psi) - \hat{\mu}^T$                      | $T_l^u$         | Location adjusted $T(\psi)$ , unconstrained bootstrap           |
| $T(\psi) - \tilde{\mu}^T$                    | $T_l^c$         | Location adjusted $T(\psi)$ , constrained bootstrap             |
| $S(\psi) - \hat{\mu}^S$                      | $S_l^u$         | Location adjusted $S(\psi)$ , unconstrained bootstrap           |
| $S(\psi) - \tilde{\mu}^S$                    | $S_l^c$         | Location adjusted $S(\psi)$ , constrained bootstrap             |
| $R(\psi) - \hat{\mu}^R$                      | $R_l^u$         | Location adjusted $R(\psi)$ , unconstrained bootstrap           |
| $R(\psi) - \tilde{\mu}^R$                    | $R_l^c$         | Location adjusted $R(\psi)$ , constrained bootstrap             |
| $(T(\psi) - \hat{\mu}^T)/\tilde{\sigma}^T$   | $T_{ls}^u$      | Location-and-scale adjusted $T(\psi)$ , unconstrained bootstrap |
| $(T(\psi) - \tilde{\mu}^T)/\tilde{\sigma}^T$ | $T_{ls}^c$      | Location-and-scale adjusted $T(\psi)$ , constrained bootstrap   |
| $(S(\psi) - \hat{\mu}^S)/\tilde{\sigma}^S$   | $S_{ls}^u$      | Location-and-scale adjusted $S(\psi)$ , unconstrained bootstrap |
| $(S(\psi) - \tilde{\mu}^S)/\tilde{\sigma}^S$ | $S_{ls}^c$      | Location-and-scale adjusted $S(\psi)$ , constrained bootstrap   |
| $(R(\psi) - \hat{\mu}^R)/\tilde{\sigma}^R$   | $R_{ls}^u$      | Location-and-scale adjusted $R(\psi)$ , unconstrained bootstrap |
| $(R(\psi) - \tilde{\mu}^R)/\tilde{\sigma}^R$ | $R_{ls}^c$      | Location-and-scale adjusted $R(\psi)$ , constrained bootstrap   |

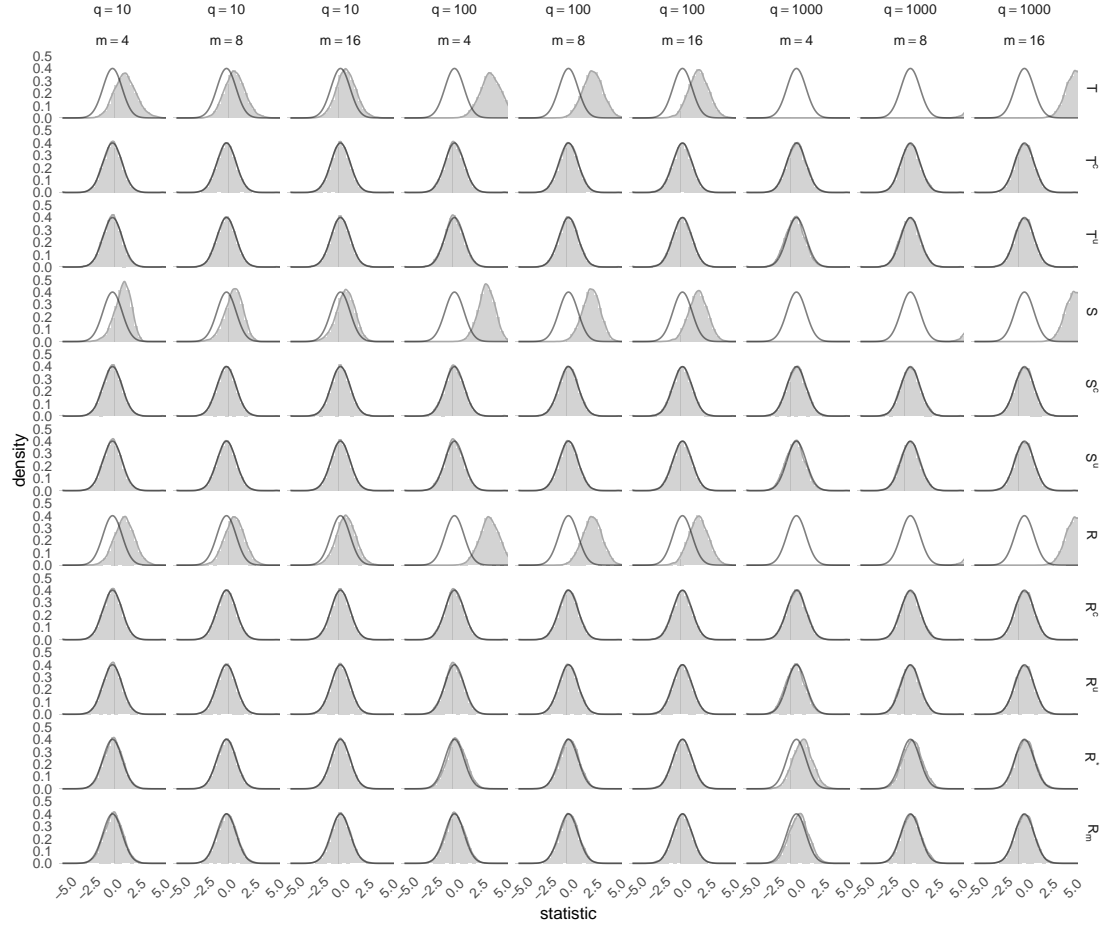

Figure S1: Gamma model. Estimated null distribution of statistics for the statistics in Table S1 for various combinations of  $q$  and  $m$ . The  $N(0,1)$  density function is superimposed.

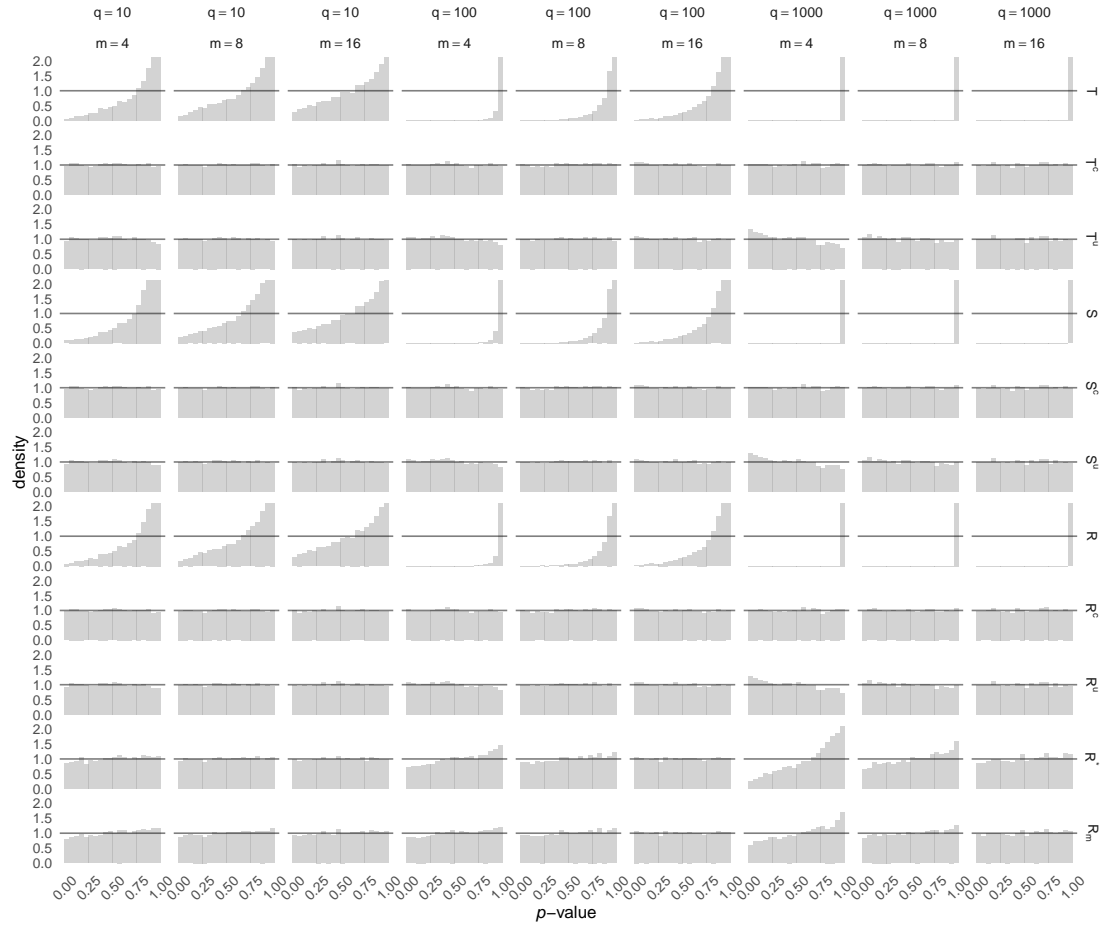

Figure S2: Gamma model. Estimated distribution of  $p$ -values for the statistics in Table S1 for various combinations of  $q$  and  $m$ . The Uniform(0,1) density function is superimposed.

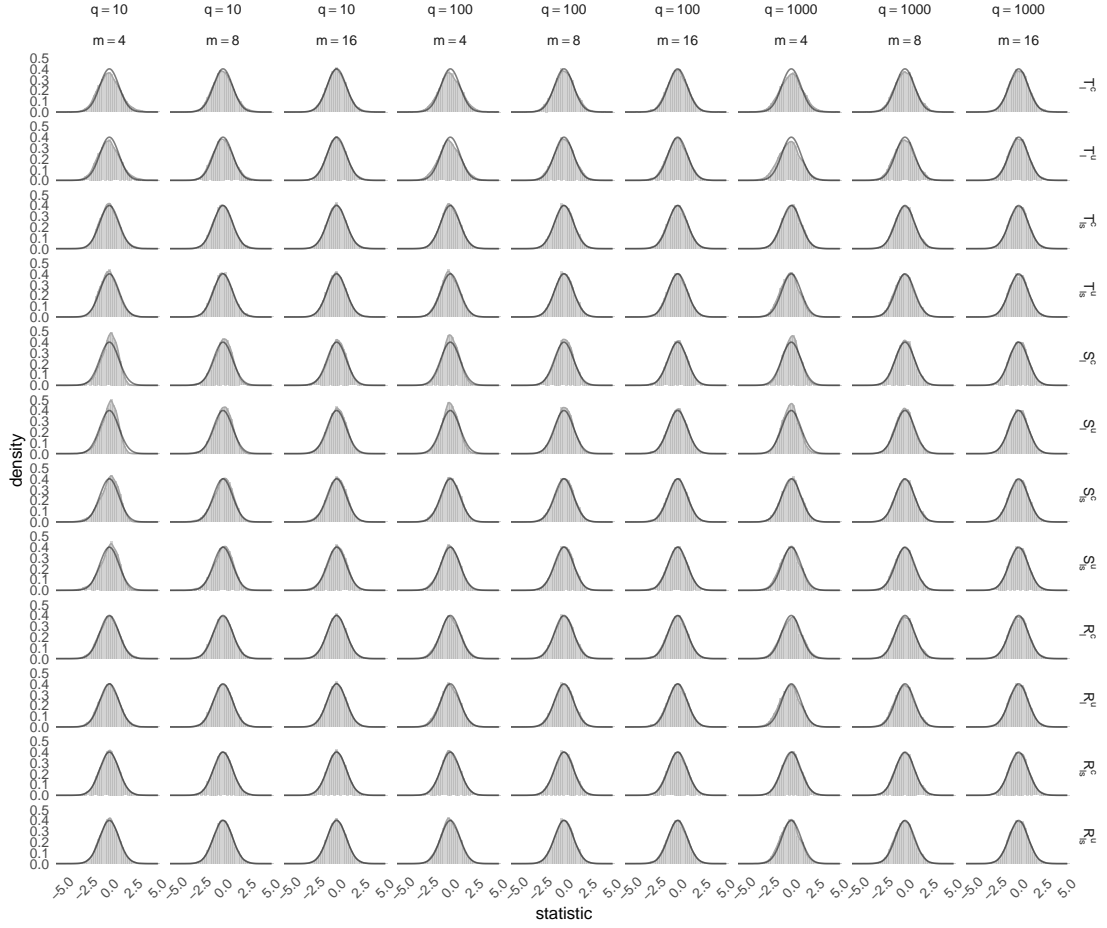

Figure S3: Gamma model. Estimated null distribution of statistics for the statistics in Table S2 for various combinations of  $q$  and  $m$ . The  $N(0,1)$  density function is superimposed.

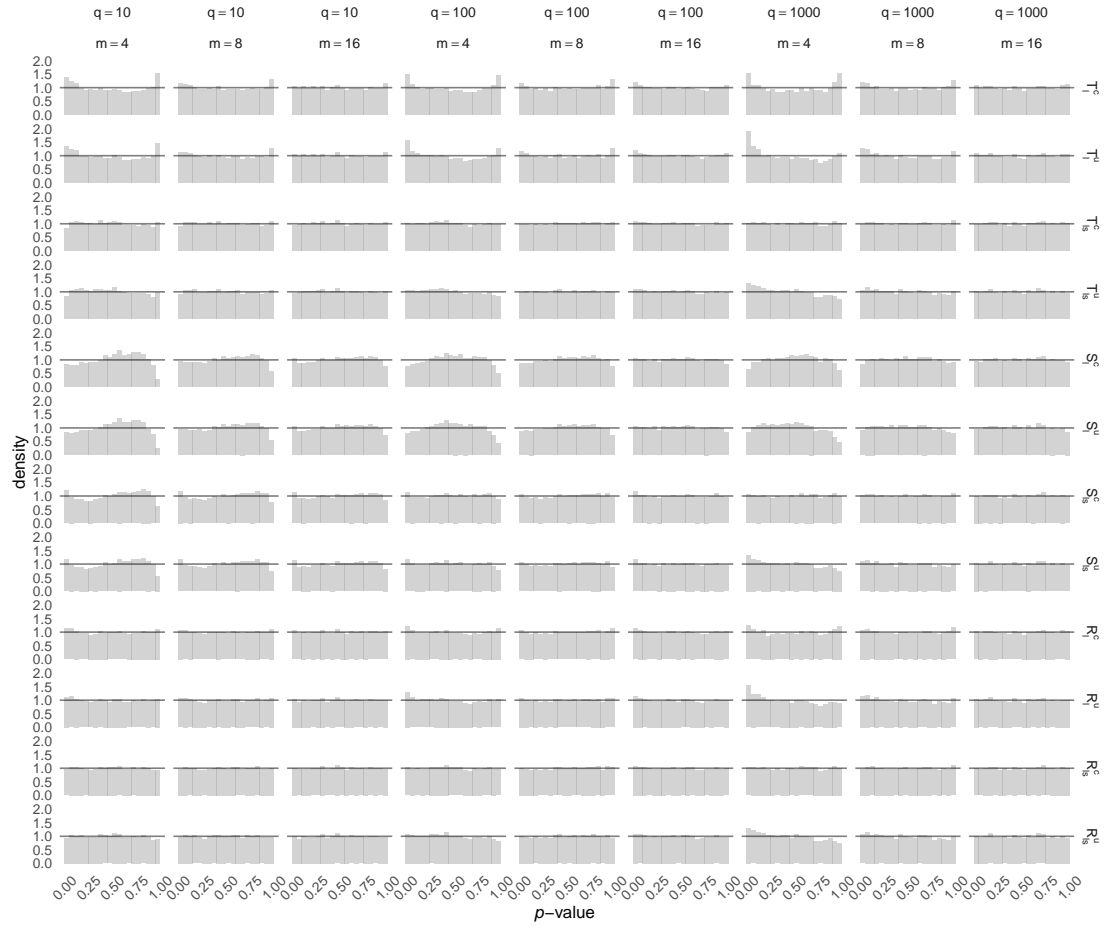

Figure S4: Gamma model. Estimated null distribution of  $p$ -values for the statistics in Table S2 for various combinations of  $q$  and  $m$ . The Uniform(0,1) density function is superimposed.

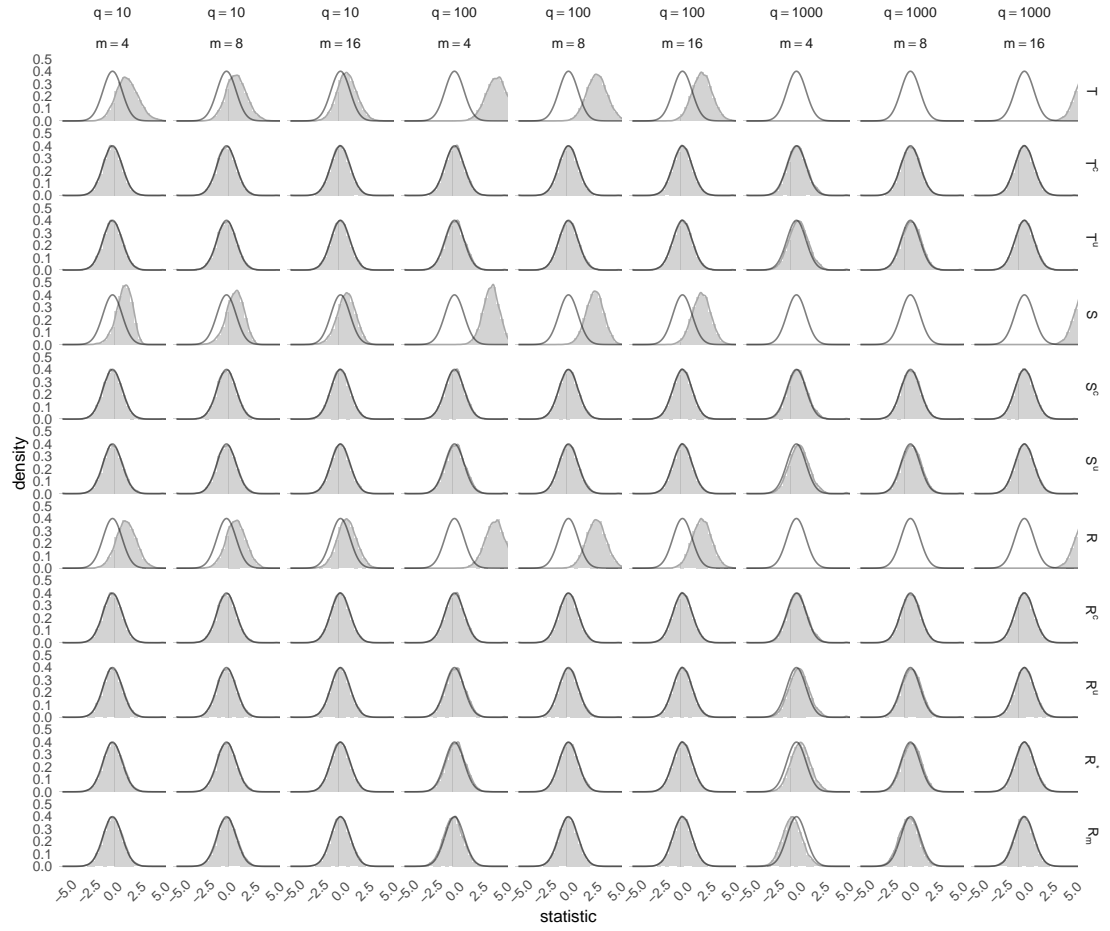

Figure S5: Beta model. Estimated null distribution of statistics for the statistics in Table S1 for various combinations of  $q$  and  $m$ . The  $N(0,1)$  density function is superimposed.

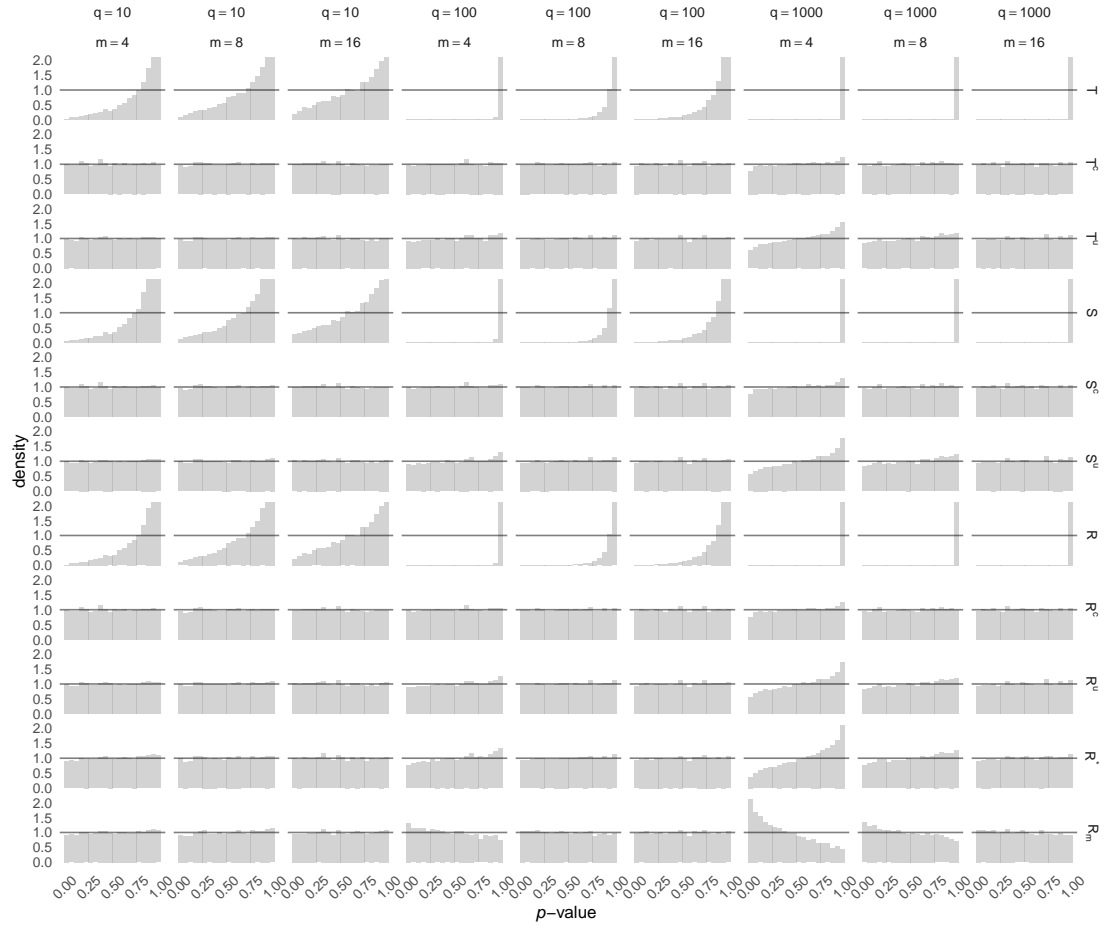

Figure S6: Beta model. Estimated distribution of  $p$ -values for the statistics in Table S1 for various combinations of  $q$  and  $m$ . The Uniform(0,1) density function is superimposed.

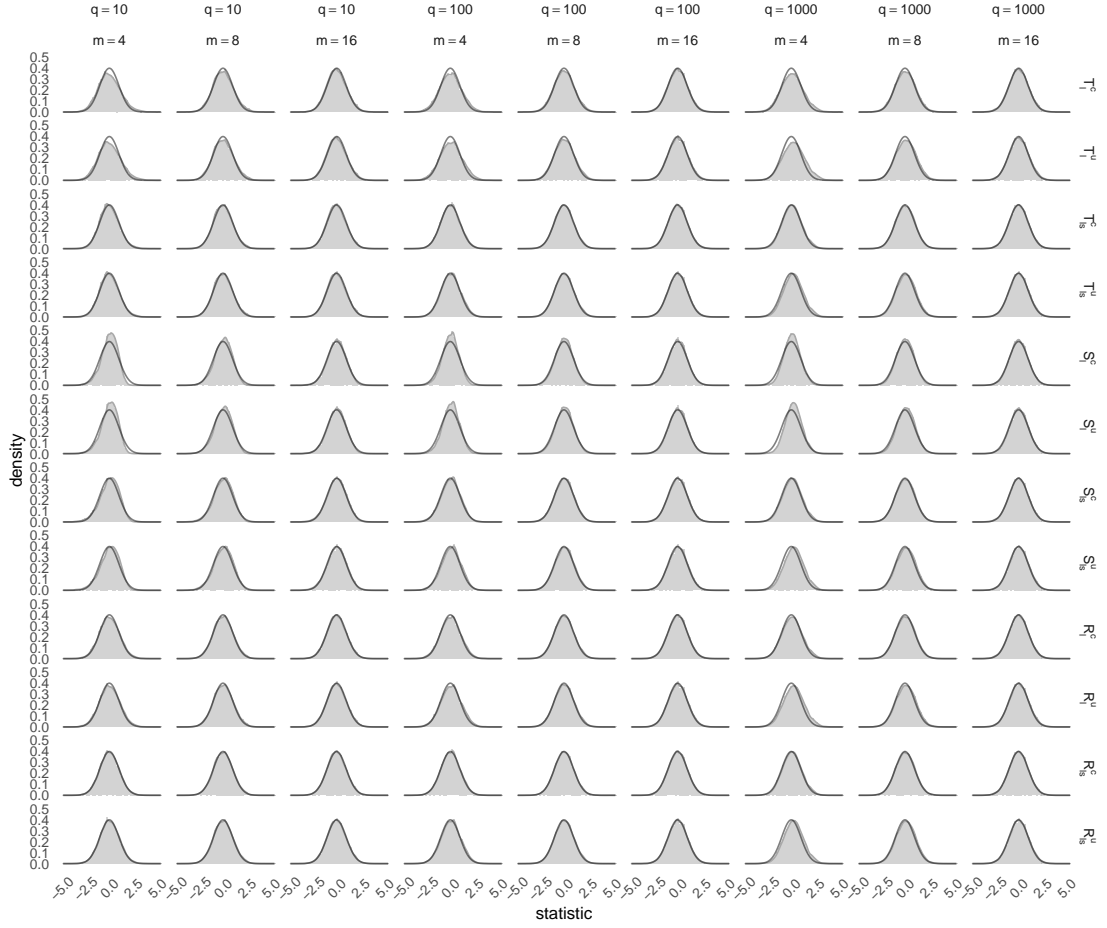

Figure S7: Beta model. Estimated null distribution of statistics for the statistics in Table S2 for various combinations of  $q$  and  $m$ . The  $N(0,1)$  density function is superimposed.

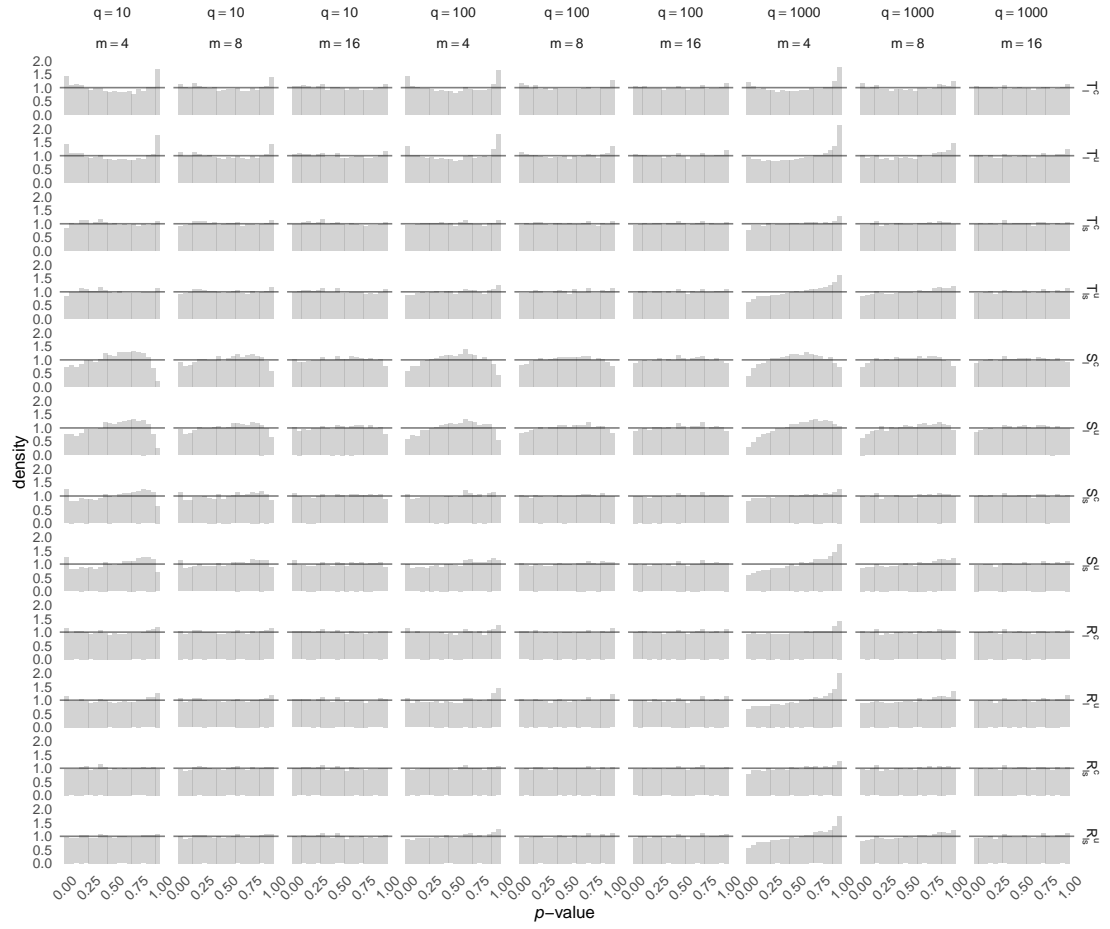

Figure S8: Beta model. Estimated null distribution of  $p$ -values for the statistics in Table S2 for various combinations of  $q$  and  $m$ . The Uniform(0,1) density function is superimposed.

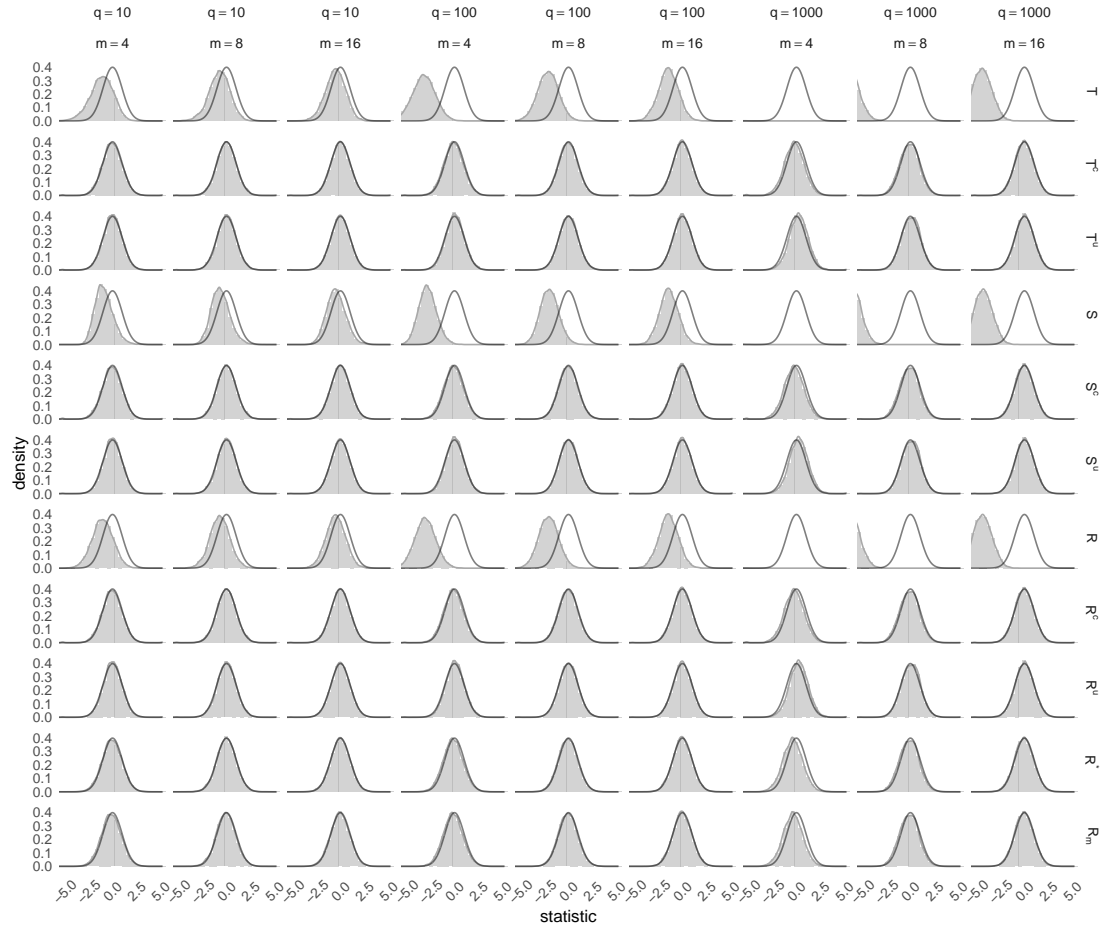

Figure S9: Curved exponential family. Estimated null distribution of statistics for the statistics in Table S1 for various combinations of  $q$  and  $m$ . The  $N(0,1)$  density function is superimposed.

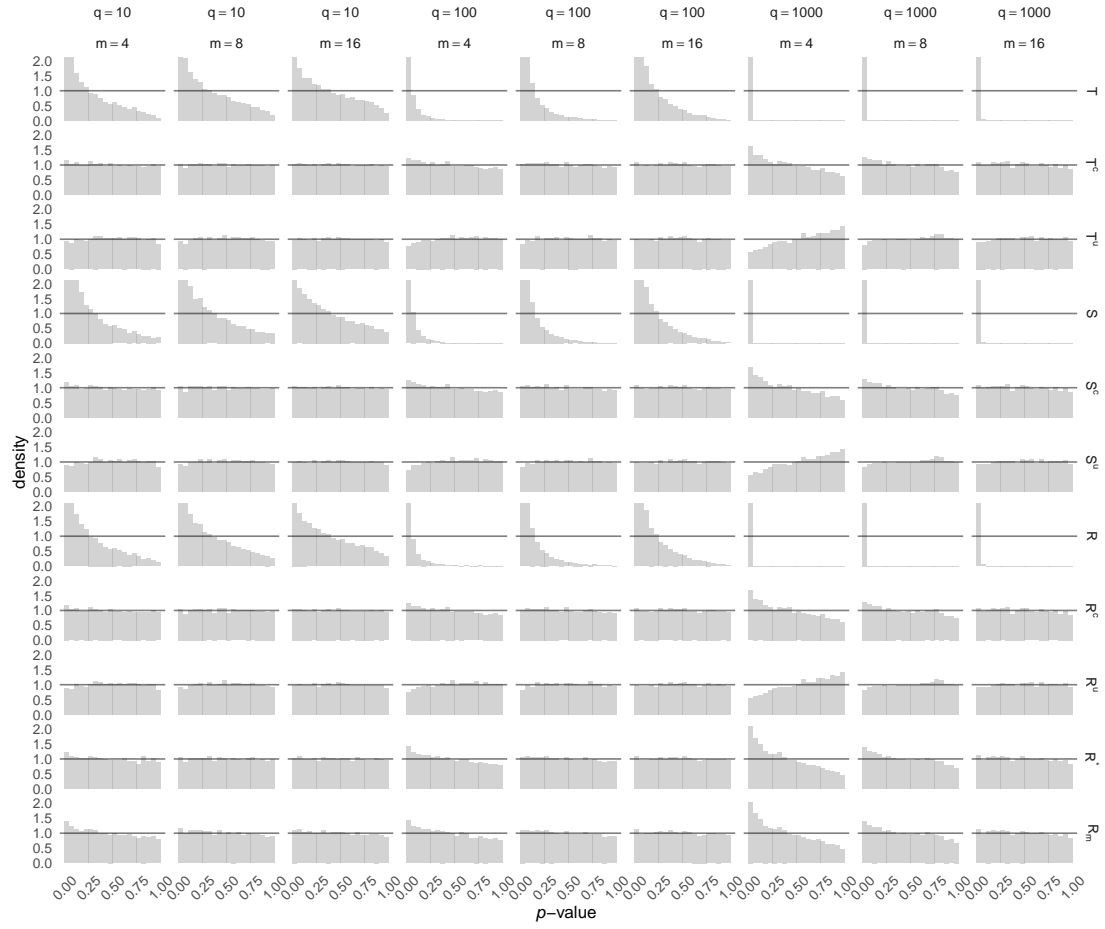

Figure S10: Curved exponential family. Estimated distribution of  $p$ -values for the statistics in Table S1 for various combinations of  $q$  and  $m$ . The Uniform(0,1) density function is superimposed.

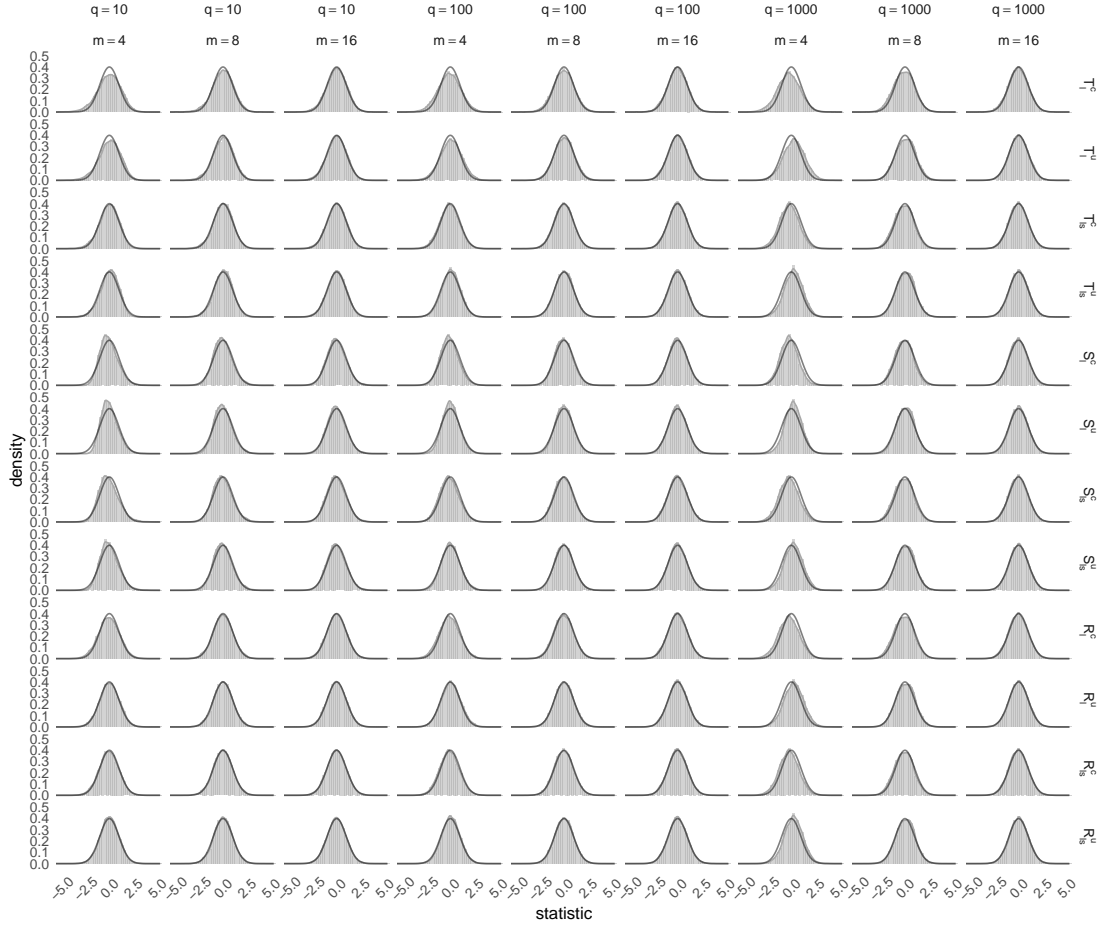

Figure S11: Curved exponential family. Estimated null distribution of statistics for the statistics in Table S2 for various combinations of  $q$  and  $m$ . The  $N(0,1)$  density function is superimposed.

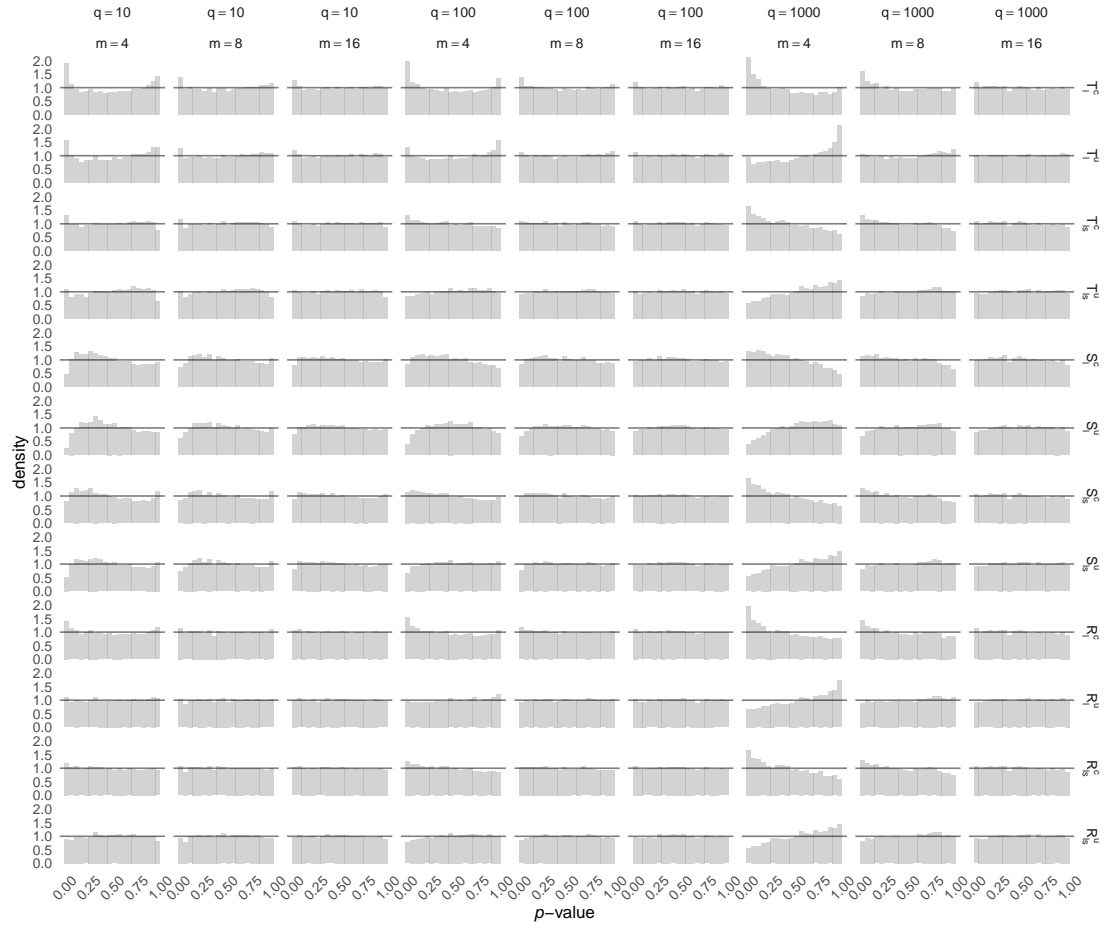

Figure S12: Curved exponential family. Estimated null distribution of  $p$ -values for the statistics in Table S2 for various combinations of  $q$  and  $m$ . The Uniform(0,1) density function is superimposed.

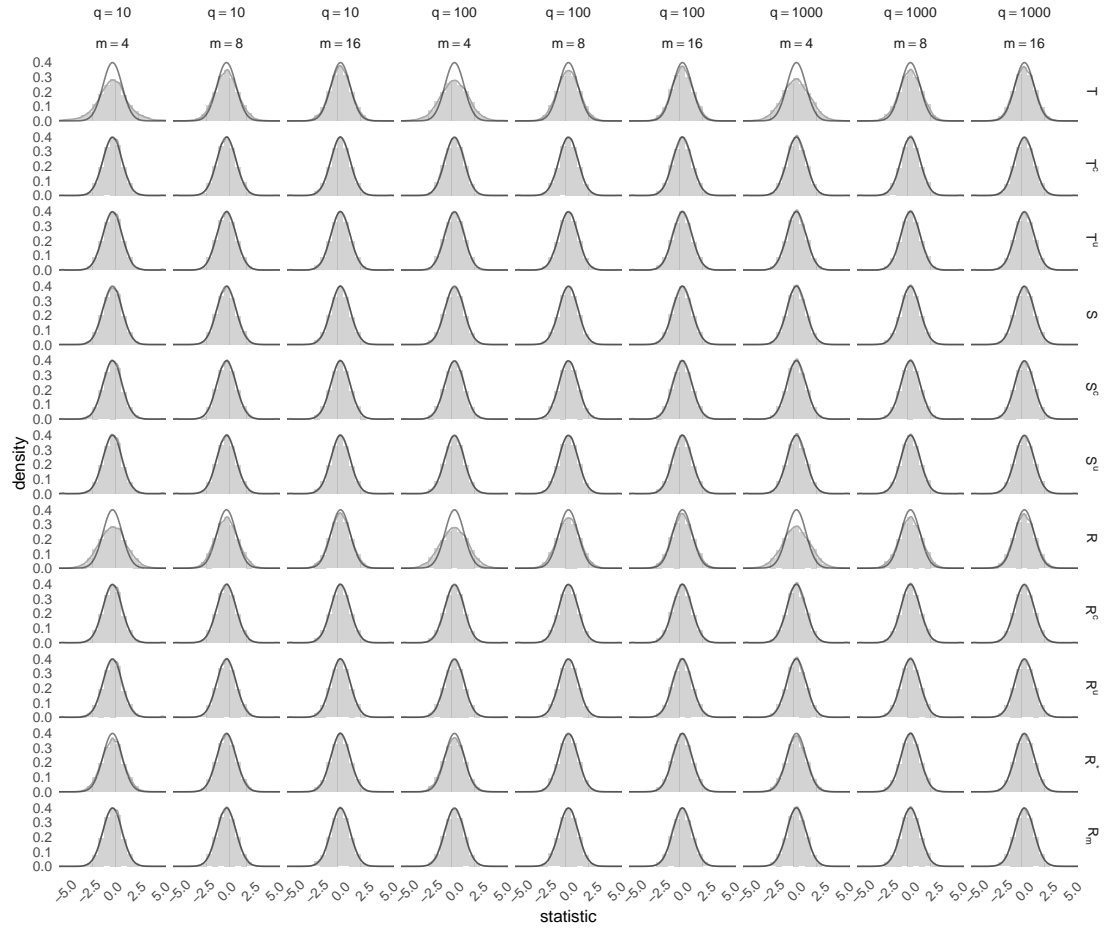

Figure S13: Behrens-Fisher model. Estimated null distribution of statistics for the statistics in Table S1 for various combinations of  $q$  and  $m$ . The  $N(0,1)$  density function is superimposed.

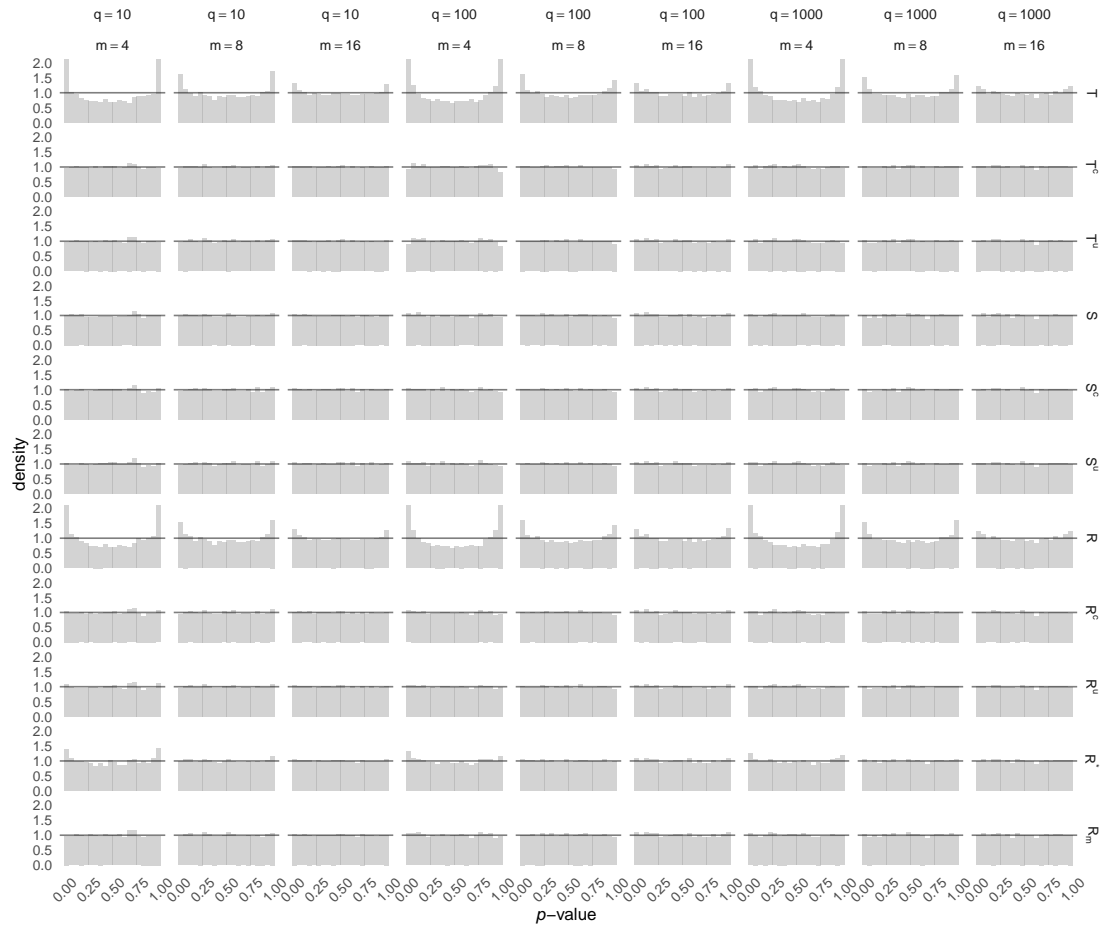

Figure S14: Behrens-Fisher model. Estimated distribution of  $p$ -values for the statistics in Table S1 for various combinations of  $q$  and  $m$ . The Uniform(0,1) density function is superimposed.

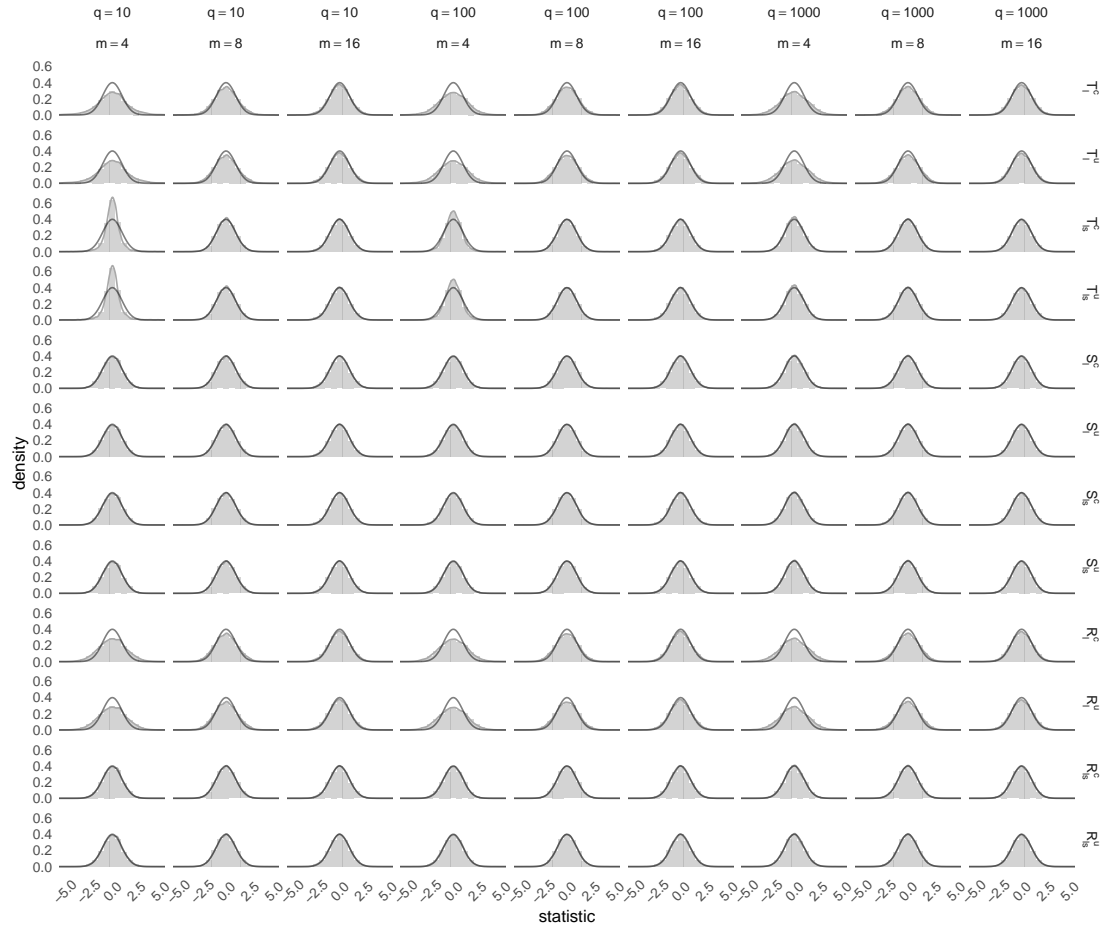

Figure S15: Behrens-Fisher model. Estimated null distribution of statistics for the statistics in Table S2 for various combinations of  $q$  and  $m$ . The  $N(0,1)$  density function is superimposed.

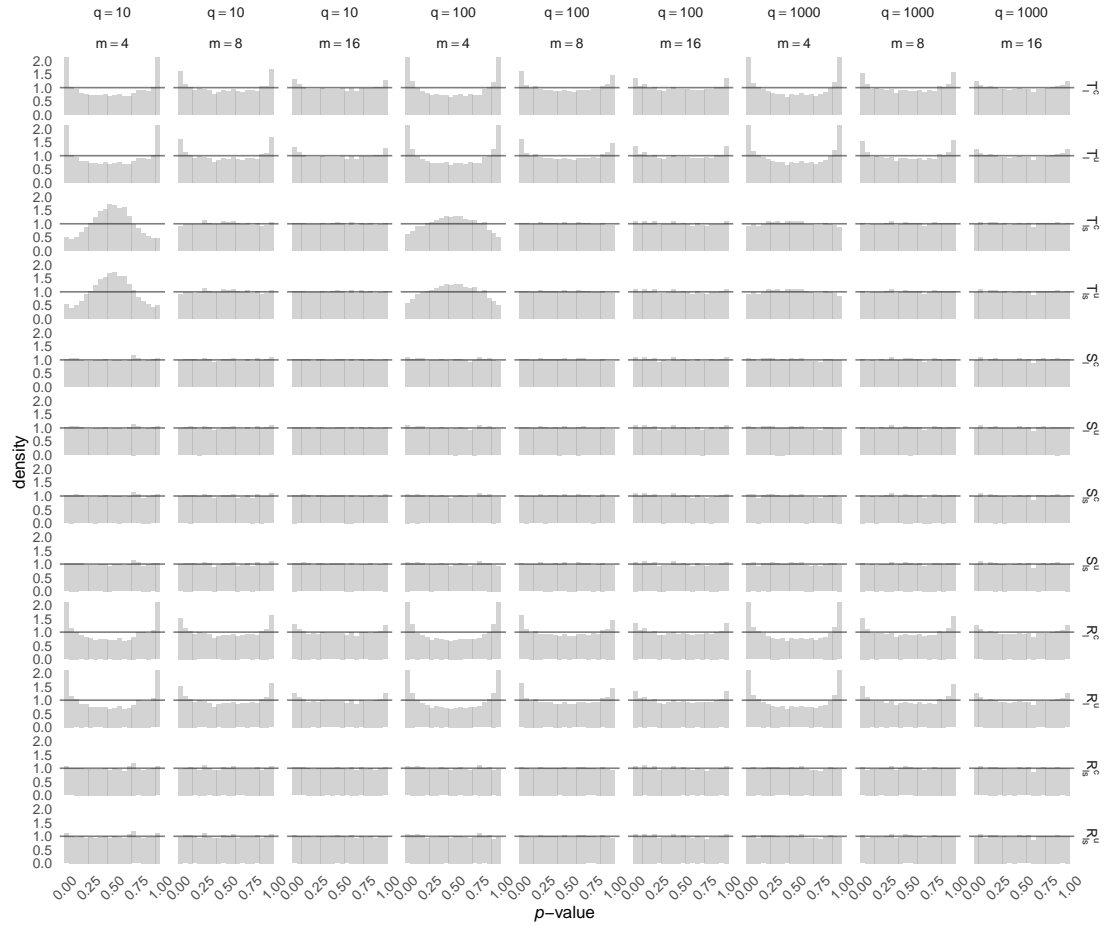

Figure S16: Behrens-Fisher model. Estimated null distribution of  $p$ -values for the statistics in Table S2 for various combinations of  $q$  and  $m$ . The Uniform(0,1) density function is superimposed.

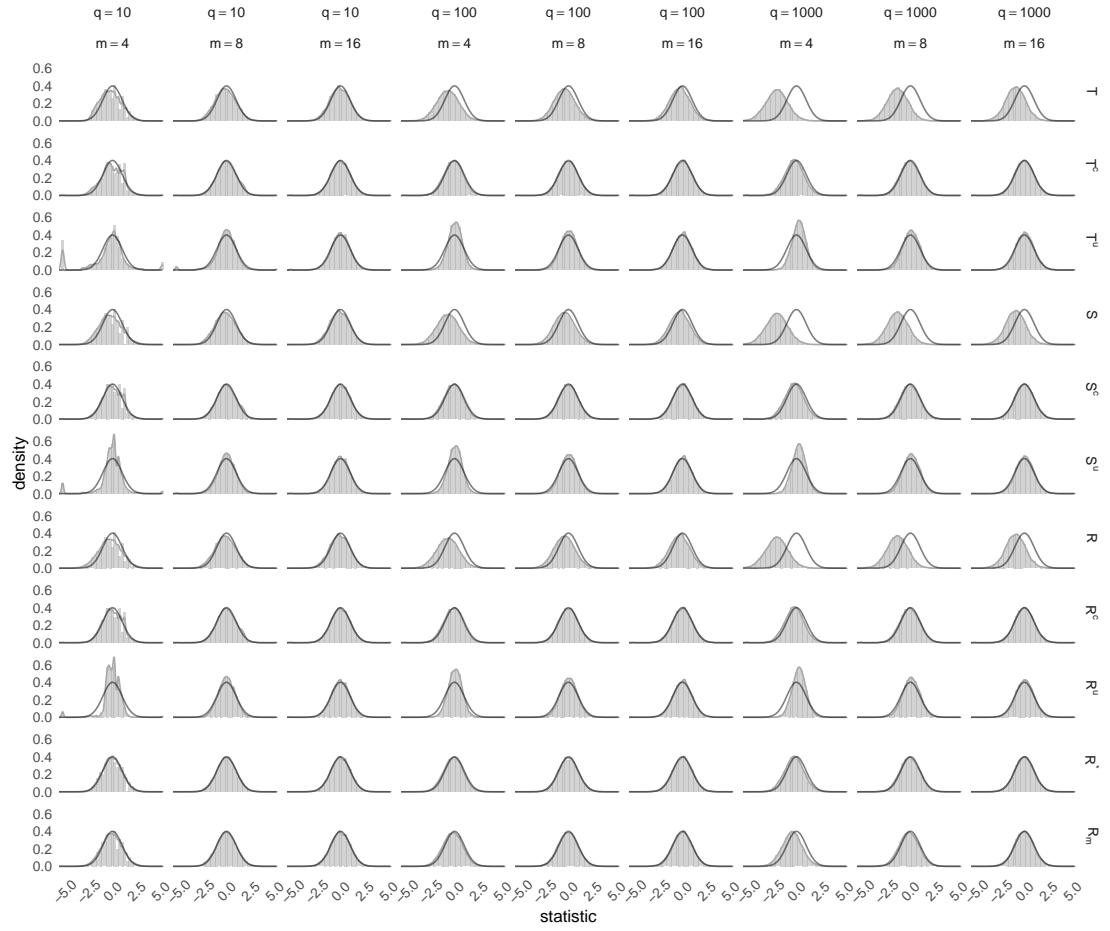

Figure S17: Logistic regression example. Estimated null distribution of statistics for the statistics in Table S1 for various combinations of  $q$  and  $m$ . The  $N(0,1)$  density function is superimposed.

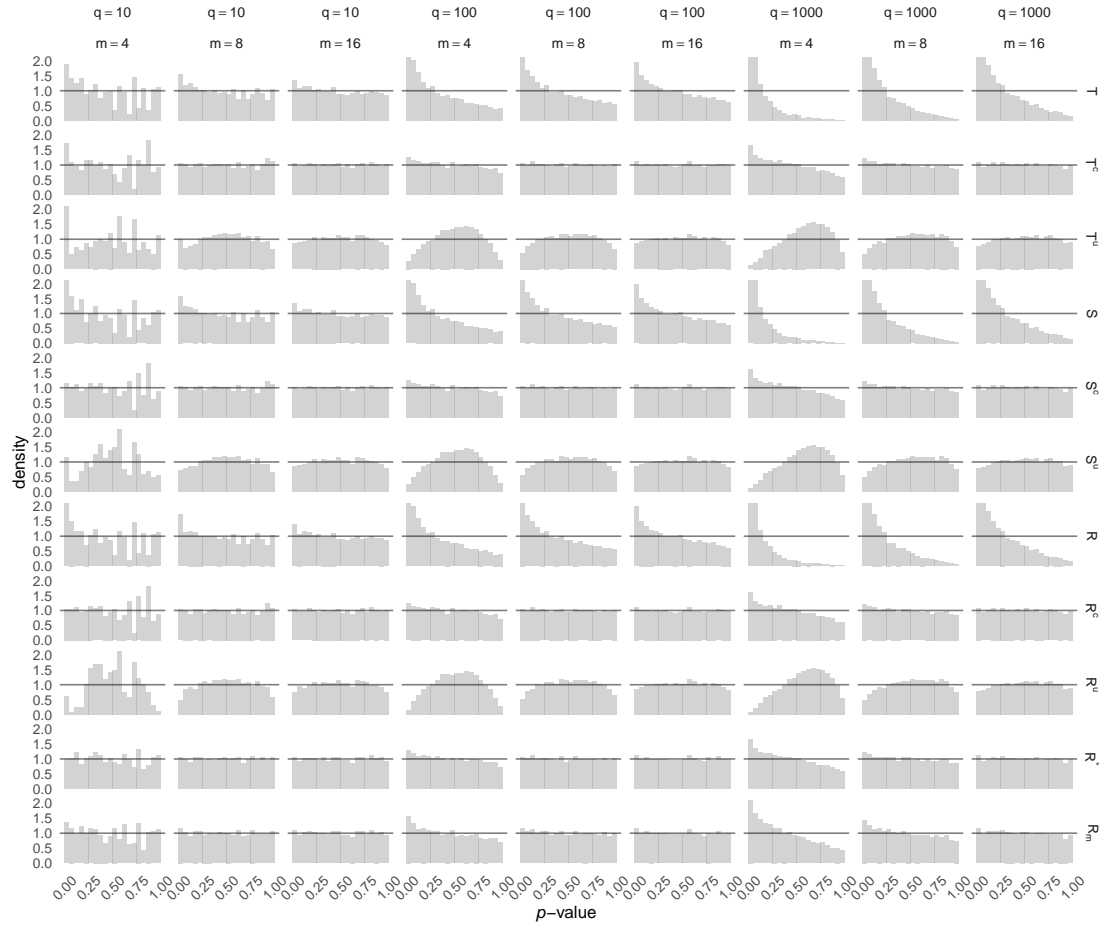

Figure S18: Logistic regression example. Estimated distribution of  $p$ -values for the statistics in Table S1 for various combinations of  $q$  and  $m$ . The Uniform(0,1) density function is superimposed.

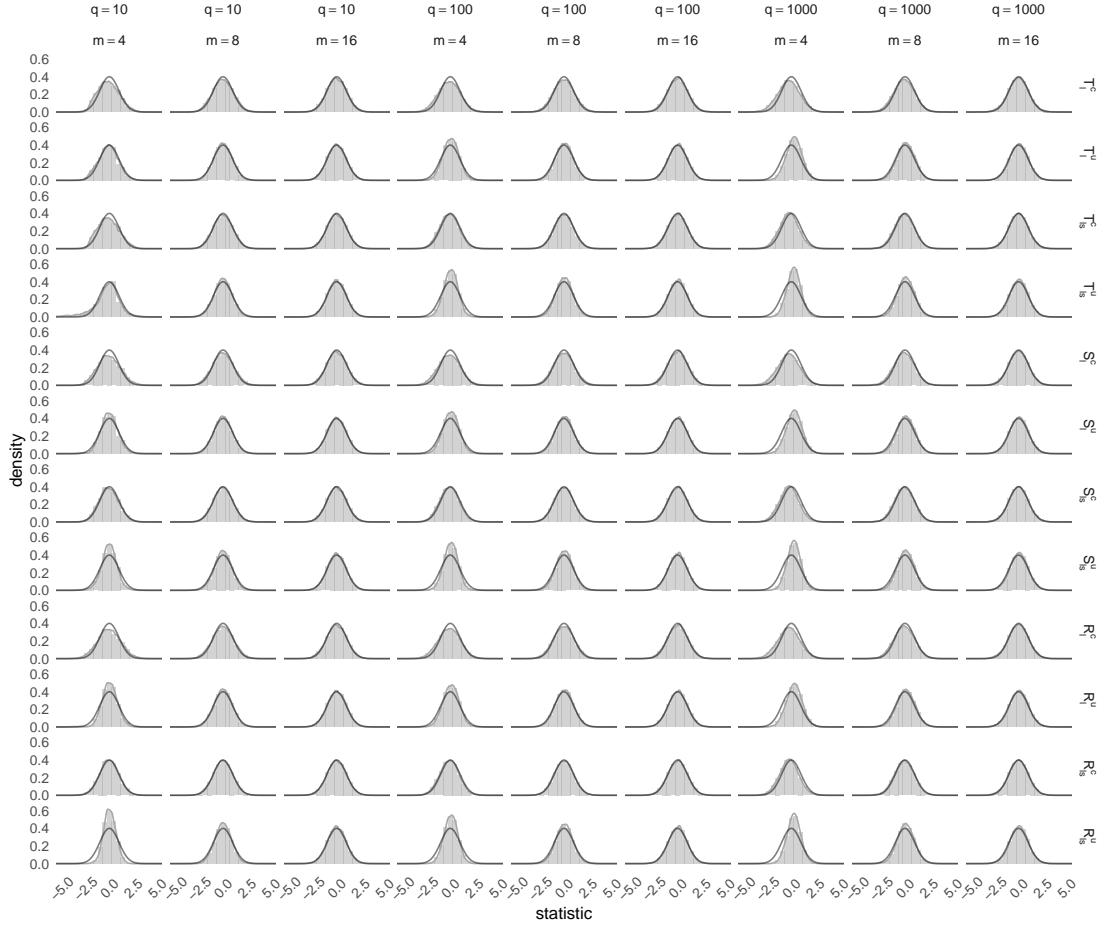

Figure S19: Logistic regression example. Estimated null distribution of statistics for the statistics in Table S2 for various combinations of  $q$  and  $m$ . The  $N(0,1)$  density function is superimposed.

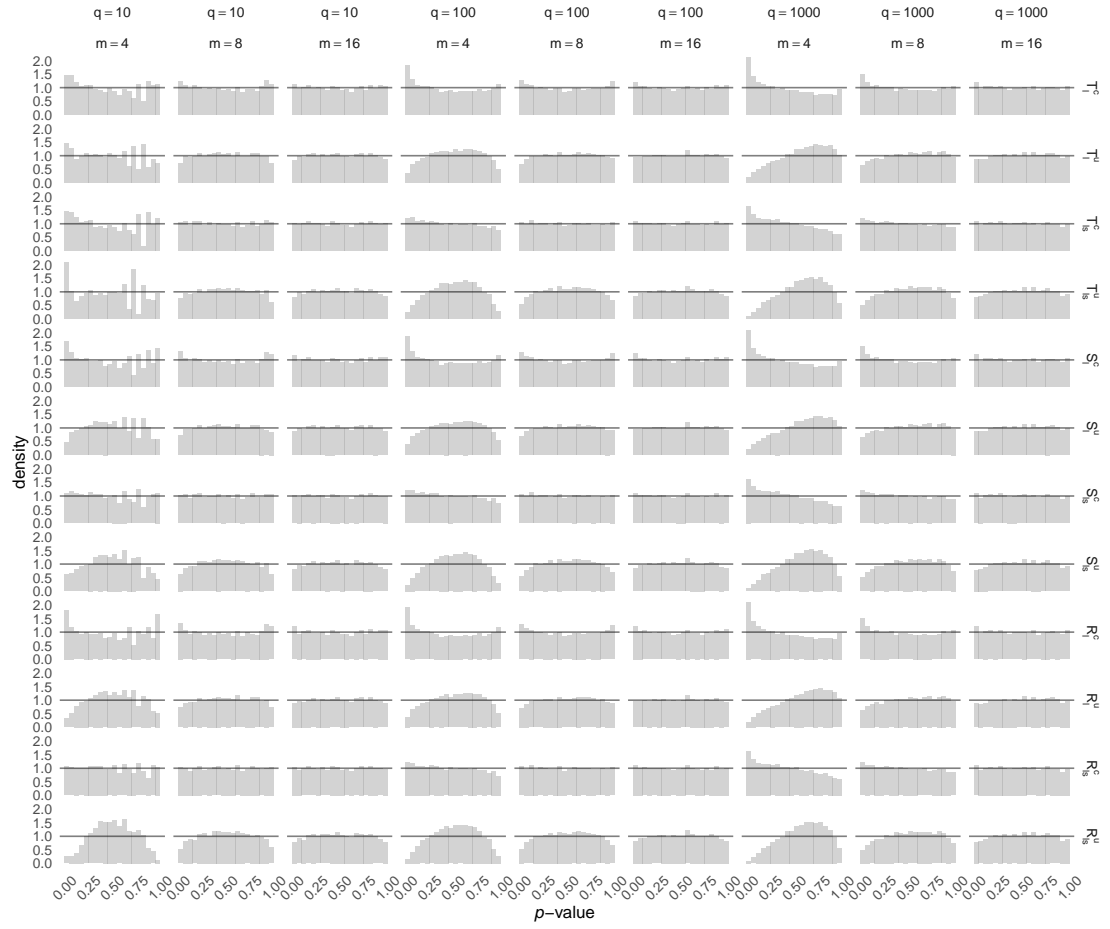

Figure S20: Logistic regression example. Estimated null distribution of  $p$ -values for the statistics in Table S2 for various combinations of  $q$  and  $m$ . The Uniform(0,1) density function is superimposed.

## Empirical tail probabilities

The following tables report empirical tail probabilities for the statistics in Table 1 of the main text, for all models and all simulation settings. The rows of each table are subdivided into 5 different blocks, each one corresponding to a different model.

Table S3: Empirical tail probabilities  $\times 100$  for the statistics in Table 1 of the main text and all models that have been considered in the simulation experiments. The figures shown have been rounded to 1 decimal and are for  $q = 10$  and  $m = 4$ .

| Model                     | Statistic  | Nominal |      |      |      |      |      |
|---------------------------|------------|---------|------|------|------|------|------|
|                           |            | 1.0     | 2.5  | 5.0  | 95.0 | 97.5 | 99.0 |
| Gamma                     | $R$        | 0.1     | 0.1  | 0.3  | 65.2 | 75.6 | 85.3 |
|                           | $R^*$      | 0.8     | 2.2  | 4.3  | 94.5 | 97.1 | 98.8 |
|                           | $R^u$      | 1.0     | 2.5  | 4.7  | 95.6 | 97.7 | 99.2 |
|                           | $R^c$      | 1.0     | 2.5  | 4.8  | 95.3 | 97.7 | 99.0 |
|                           | $R_l^c$    | 1.5     | 3.1  | 5.6  | 94.4 | 96.9 | 98.7 |
|                           | $R_{ls}^c$ | 1.0     | 2.5  | 4.8  | 95.3 | 97.5 | 99.0 |
| Beta                      | $R$        | 0.0     | 0.0  | 0.1  | 58.5 | 69.3 | 80.1 |
|                           | $R^*$      | 0.9     | 2.1  | 4.5  | 94.6 | 97.1 | 98.7 |
|                           | $R^u$      | 1.0     | 2.4  | 5.0  | 94.7 | 97.2 | 98.8 |
|                           | $R^c$      | 0.9     | 2.4  | 4.9  | 95.1 | 97.5 | 99.0 |
|                           | $R_l^c$    | 1.2     | 2.8  | 5.8  | 94.2 | 96.8 | 98.5 |
|                           | $R_{ls}^c$ | 0.9     | 2.3  | 4.9  | 95.1 | 97.5 | 98.9 |
| Curved exponential family | $R$        | 11.8    | 19.4 | 28.1 | 99.4 | 99.8 | 99.9 |
|                           | $R^*$      | 1.4     | 3.2  | 6.1  | 95.6 | 97.6 | 99.0 |
|                           | $R^u$      | 0.8     | 2.1  | 4.4  | 95.8 | 98.0 | 99.2 |
|                           | $R^c$      | 1.4     | 3.0  | 5.9  | 95.3 | 97.6 | 99.0 |
|                           | $R_l^c$    | 1.9     | 4.1  | 7.1  | 94.2 | 96.9 | 98.6 |
|                           | $R_{ls}^c$ | 1.4     | 3.1  | 6.0  | 95.4 | 97.6 | 99.0 |
| Behrens-Fisher            | $R$        | 4.9     | 8.0  | 12.1 | 88.0 | 91.8 | 95.1 |
|                           | $R^*$      | 1.9     | 4.0  | 7.0  | 92.9 | 96.0 | 98.1 |
|                           | $R^u$      | 1.4     | 2.9  | 5.4  | 94.4 | 97.0 | 98.8 |
|                           | $R^c$      | 1.1     | 2.7  | 5.2  | 94.7 | 97.3 | 98.9 |
|                           | $R_l^c$    | 4.9     | 7.9  | 12.1 | 87.9 | 91.8 | 95.1 |
|                           | $R_{ls}^c$ | 1.0     | 2.6  | 5.3  | 94.7 | 97.4 | 99.0 |
| Logistic regression       | $R$        | 3.8     | 7.1  | 12.5 | 94.4 | 97.0 | 98.4 |
|                           | $R^*$      | 0.5     | 2.2  | 5.0  | 94.4 | 97.1 | 98.7 |
|                           | $R^u$      | 2.1     | 2.6  | 3.1  | 99.4 | 99.6 | 99.7 |
|                           | $R^c$      | 0.8     | 2.4  | 5.2  | 95.6 | 97.6 | 99.0 |
|                           | $R_l^c$    | 2.9     | 5.5  | 9.1  | 91.7 | 94.5 | 97.2 |
|                           | $R_{ls}^c$ | 1.0     | 2.6  | 5.3  | 94.8 | 97.3 | 99.0 |

Table S4: Empirical tail probabilities  $\times 100$  for the statistics in Table 1 of the main text and all models that have been considered in the simulation experiments. The figures shown have been rounded to 1 decimal and are for  $q = 10$  and  $m = 8$ .

| Model                     | Statistic  | Nominal |      |      |      |      |      |
|---------------------------|------------|---------|------|------|------|------|------|
|                           |            | 1.0     | 2.5  | 5.0  | 95.0 | 97.5 | 99.0 |
| Gamma                     | $R$        | 0.1     | 0.3  | 0.9  | 78.6 | 86.5 | 92.8 |
|                           | $R^*$      | 0.9     | 2.3  | 4.6  | 94.7 | 97.4 | 98.8 |
|                           | $R^u$      | 1.0     | 2.4  | 4.9  | 95.2 | 97.7 | 99.1 |
|                           | $R^c$      | 1.0     | 2.5  | 4.9  | 95.0 | 97.5 | 99.0 |
|                           | $R_l^c$    | 1.2     | 2.8  | 5.4  | 94.4 | 97.2 | 98.7 |
|                           | $R_{ls}^c$ | 1.0     | 2.5  | 4.9  | 95.0 | 97.5 | 98.9 |
| Beta                      | $R$        | 0.1     | 0.2  | 0.5  | 73.8 | 82.8 | 90.5 |
|                           | $R^*$      | 0.9     | 2.3  | 4.9  | 94.7 | 97.1 | 98.9 |
|                           | $R^u$      | 0.9     | 2.4  | 4.9  | 94.5 | 97.1 | 98.8 |
|                           | $R^c$      | 0.9     | 2.4  | 4.8  | 94.8 | 97.4 | 99.0 |
|                           | $R_l^c$    | 1.0     | 2.6  | 5.2  | 94.4 | 96.9 | 98.8 |
|                           | $R_{ls}^c$ | 0.9     | 2.3  | 4.9  | 94.8 | 97.2 | 98.9 |
| Curved exponential family | $R$        | 5.8     | 10.5 | 17.4 | 98.8 | 99.5 | 99.8 |
|                           | $R^*$      | 1.1     | 3.0  | 5.3  | 95.1 | 97.5 | 99.0 |
|                           | $R^u$      | 0.9     | 2.3  | 4.5  | 95.4 | 97.7 | 99.3 |
|                           | $R^c$      | 1.1     | 2.9  | 5.2  | 95.0 | 97.4 | 99.1 |
|                           | $R_l^c$    | 1.3     | 3.3  | 5.8  | 94.5 | 97.1 | 98.8 |
|                           | $R_{ls}^c$ | 1.1     | 3.0  | 5.3  | 95.0 | 97.4 | 99.1 |
| Behrens-Fisher            | $R$        | 2.0     | 4.3  | 7.6  | 92.0 | 95.2 | 97.6 |
|                           | $R^*$      | 1.0     | 2.5  | 5.0  | 94.3 | 97.0 | 99.0 |
|                           | $R^u$      | 1.0     | 2.3  | 4.8  | 94.5 | 97.3 | 99.1 |
|                           | $R^c$      | 1.0     | 2.3  | 4.8  | 94.5 | 97.3 | 99.2 |
|                           | $R_l^c$    | 2.0     | 4.3  | 7.6  | 91.9 | 95.2 | 97.6 |
|                           | $R_{ls}^c$ | 0.9     | 2.4  | 4.9  | 94.5 | 97.2 | 99.0 |
| Logistic regression       | $R$        | 2.2     | 4.7  | 8.6  | 94.8 | 97.0 | 99.1 |
|                           | $R^*$      | 0.9     | 2.7  | 5.3  | 94.8 | 97.0 | 99.1 |
|                           | $R^u$      | 0.1     | 0.7  | 2.4  | 97.2 | 98.9 | 99.6 |
|                           | $R^c$      | 0.9     | 2.6  | 5.2  | 94.5 | 97.9 | 99.1 |
|                           | $R_l^c$    | 1.6     | 3.6  | 6.7  | 94.0 | 96.9 | 98.4 |
|                           | $R_{ls}^c$ | 0.9     | 2.6  | 5.2  | 94.8 | 97.4 | 99.0 |

Table S5: Empirical tail probabilities  $\times 100$  for the statistics in Table 1 of the main text and all models that have been considered in the simulation experiments. The figures shown have been rounded to 1 decimal and are for  $q = 10$  and  $m = 16$ .

| Model                     | Statistic  | Nominal |     |      |      |      |      |
|---------------------------|------------|---------|-----|------|------|------|------|
|                           |            | 1.0     | 2.5 | 5.0  | 95.0 | 97.5 | 99.0 |
| Gamma                     | $R$        | 0.2     | 0.6 | 1.5  | 85.7 | 91.6 | 96.0 |
|                           | $R^*$      | 1.1     | 2.5 | 4.9  | 95.0 | 97.4 | 98.9 |
|                           | $R^u$      | 1.0     | 2.6 | 5.0  | 95.2 | 97.5 | 99.0 |
|                           | $R^c$      | 1.1     | 2.6 | 5.1  | 95.1 | 97.5 | 99.0 |
|                           | $R_l^c$    | 1.2     | 2.8 | 5.3  | 94.9 | 97.3 | 98.9 |
|                           | $R_{ls}^c$ | 1.2     | 2.6 | 5.1  | 95.1 | 97.4 | 98.9 |
| Beta                      | $R$        | 0.2     | 0.4 | 1.1  | 83.4 | 89.8 | 94.8 |
|                           | $R^*$      | 1.0     | 2.4 | 5.0  | 94.9 | 97.5 | 99.1 |
|                           | $R^u$      | 1.1     | 2.6 | 5.1  | 94.8 | 97.4 | 99.0 |
|                           | $R^c$      | 1.0     | 2.4 | 5.0  | 95.0 | 97.5 | 99.1 |
|                           | $R_l^c$    | 1.0     | 2.5 | 5.1  | 94.9 | 97.3 | 99.0 |
|                           | $R_{ls}^c$ | 1.0     | 2.4 | 5.0  | 95.0 | 97.5 | 99.1 |
| Curved exponential family | $R$        | 3.7     | 7.7 | 13.1 | 98.4 | 99.2 | 99.8 |
|                           | $R^*$      | 1.1     | 2.7 | 5.1  | 95.3 | 97.8 | 99.1 |
|                           | $R^u$      | 1.0     | 2.4 | 4.9  | 95.5 | 97.9 | 99.2 |
|                           | $R^c$      | 1.1     | 2.6 | 5.2  | 95.3 | 97.8 | 99.1 |
|                           | $R_l^c$    | 1.3     | 3.3 | 5.8  | 94.5 | 97.1 | 98.8 |
|                           | $R_{ls}^c$ | 1.1     | 3.0 | 5.3  | 95.0 | 97.4 | 99.1 |
| Behrens-Fisher            | $R$        | 1.8     | 3.5 | 6.4  | 93.7 | 96.7 | 98.6 |
|                           | $R^*$      | 1.2     | 2.9 | 5.3  | 94.8 | 97.4 | 99.0 |
|                           | $R^u$      | 1.2     | 2.8 | 5.2  | 94.9 | 97.5 | 99.1 |
|                           | $R^c$      | 1.2     | 2.8 | 5.1  | 94.9 | 97.5 | 99.1 |
|                           | $R_l^c$    | 1.8     | 3.5 | 6.4  | 93.8 | 96.6 | 98.6 |
|                           | $R_{ls}^c$ | 1.2     | 2.9 | 5.1  | 94.9 | 97.4 | 99.1 |
| Logistic regression       | $R$        | 1.7     | 3.7 | 7.0  | 95.7 | 98.0 | 99.3 |
|                           | $R^*$      | 1.0     | 2.7 | 5.2  | 95.4 | 97.7 | 99.3 |
|                           | $R^u$      | 0.6     | 1.8 | 3.8  | 96.3 | 98.4 | 99.5 |
|                           | $R^c$      | 1.0     | 2.6 | 5.1  | 94.9 | 97.5 | 99.0 |
|                           | $R_l^c$    | 1.2     | 3.1 | 6.0  | 94.6 | 97.2 | 98.9 |
|                           | $R_{ls}^c$ | 1.0     | 2.7 | 5.2  | 95.1 | 97.6 | 99.1 |

Table S6: Empirical tail probabilities  $\times 100$  for the statistics in Table 1 of the main text and all models that have been considered in the simulation experiments. The figures shown have been rounded to 1 decimal and are for  $q = 100$  and  $m = 4$ .

| Model                     | Statistic  | Nominal |      |      |       |       |       |
|---------------------------|------------|---------|------|------|-------|-------|-------|
|                           |            | 1.0     | 2.5  | 5.0  | 95.0  | 97.5  | 99.0  |
| Gamma                     | $R$        | 0.0     | 0.0  | 0.0  | 2.7   | 5.2   | 10.0  |
|                           | $R^*$      | 0.6     | 1.6  | 3.5  | 92.8  | 96.2  | 98.4  |
|                           | $R^u$      | 1.0     | 2.8  | 5.4  | 95.9  | 98.0  | 99.3  |
|                           | $R^c$      | 0.9     | 2.6  | 5.2  | 95.2  | 97.6  | 99.1  |
|                           | $R_l^c$    | 1.3     | 3.4  | 6.1  | 94.2  | 96.9  | 98.7  |
|                           | $R_{ls}^c$ | 1.0     | 2.6  | 5.2  | 95.2  | 97.5  | 99.1  |
| Beta                      | $R$        | 0.0     | 0.0  | 0.0  | 0.7   | 1.4   | 3.4   |
|                           | $R^*$      | 0.8     | 2.0  | 3.8  | 93.4  | 96.7  | 98.7  |
|                           | $R^u$      | 0.9     | 2.3  | 4.5  | 93.7  | 97.0  | 98.7  |
|                           | $R^c$      | 0.9     | 2.5  | 4.9  | 94.8  | 97.4  | 99.1  |
|                           | $R_l^c$    | 1.3     | 2.9  | 5.7  | 93.8  | 96.9  | 98.7  |
|                           | $R_{ls}^c$ | 1.0     | 2.5  | 4.9  | 94.7  | 97.5  | 99.0  |
| Curved exponential family | $R$        | 75.1    | 84.2 | 90.3 | 100.0 | 100.0 | 100.0 |
|                           | $R^*$      | 1.6     | 3.7  | 7.1  | 96.0  | 97.9  | 99.2  |
|                           | $R^u$      | 0.7     | 1.7  | 3.7  | 95.0  | 97.5  | 99.0  |
|                           | $R^c$      | 1.3     | 3.2  | 6.2  | 95.7  | 97.8  | 99.1  |
|                           | $R_l^c$    | 1.8     | 4.2  | 7.7  | 94.7  | 97.2  | 98.7  |
|                           | $R_{ls}^c$ | 1.5     | 3.3  | 6.3  | 95.7  | 97.7  | 99.1  |
| Behrens-Fisher            | $R$        | 5.2     | 8.8  | 12.8 | 88.5  | 92.2  | 95.2  |
|                           | $R^*$      | 1.7     | 3.5  | 6.7  | 94.2  | 96.8  | 98.6  |
|                           | $R^u$      | 1.2     | 2.8  | 5.3  | 95.1  | 97.7  | 98.9  |
|                           | $R^c$      | 1.1     | 2.8  | 5.3  | 95.2  | 97.7  | 99.0  |
|                           | $R_l^c$    | 5.3     | 8.9  | 12.8 | 88.4  | 92.2  | 95.3  |
|                           | $R_{ls}^c$ | 1.1     | 2.8  | 5.3  | 95.2  | 97.7  | 99.0  |
| Logistic regression       | $R$        | 8.1     | 14.0 | 20.5 | 98.0  | 99.0  | 99.5  |
|                           | $R^*$      | 1.4     | 3.2  | 6.4  | 96.4  | 98.1  | 99.2  |
|                           | $R^u$      | 0.1     | 0.2  | 0.8  | 98.6  | 99.6  | 99.9  |
|                           | $R^c$      | 1.3     | 3.2  | 6.2  | 96.4  | 98.2  | 99.2  |
|                           | $R_l^c$    | 2.8     | 5.7  | 9.5  | 94.2  | 96.8  | 98.3  |
|                           | $R_{ls}^c$ | 1.3     | 3.2  | 6.1  | 96.4  | 98.1  | 99.2  |

Table S7: Empirical tail probabilities  $\times 100$  for the statistics in Table 1 of the main text and all models that have been considered in the simulation experiments. The figures shown have been rounded to 1 decimal and are for  $q = 100$  and  $m = 8$ .

| Model                     | Statistic  | Nominal |      |      |       |       |       |
|---------------------------|------------|---------|------|------|-------|-------|-------|
|                           |            | 1.0     | 2.5  | 5.0  | 95.0  | 97.5  | 99.0  |
| Gamma                     | $R$        | 0.0     | 0.0  | 0.0  | 20.5  | 29.8  | 43.5  |
|                           | $R^*$      | 0.8     | 2.0  | 4.4  | 93.8  | 97.1  | 98.9  |
|                           | $R^u$      | 0.9     | 2.4  | 5.0  | 95.2  | 97.8  | 99.1  |
|                           | $R^c$      | 1.1     | 2.4  | 5.0  | 94.9  | 97.5  | 99.1  |
|                           | $R_l^c$    | 1.1     | 2.7  | 5.3  | 94.3  | 97.2  | 99.0  |
|                           | $R_{ls}^c$ | 1.0     | 2.5  | 5.0  | 94.9  | 97.5  | 99.1  |
| Beta                      | $R$        | 0.0     | 0.0  | 0.0  | 10.7  | 17.5  | 28.6  |
|                           | $R^*$      | 0.8     | 2.2  | 4.6  | 94.4  | 97.2  | 99.0  |
|                           | $R^u$      | 0.9     | 2.3  | 4.7  | 94.3  | 97.1  | 98.9  |
|                           | $R^c$      | 0.9     | 2.4  | 4.9  | 94.7  | 97.2  | 99.0  |
|                           | $R_l^c$    | 1.1     | 2.6  | 5.2  | 94.4  | 97.1  | 98.9  |
|                           | $R_{ls}^c$ | 0.9     | 2.4  | 4.9  | 94.7  | 97.4  | 99.0  |
| Curved exponential family | $R$        | 40.6    | 54.4 | 66.0 | 100.0 | 100.0 | 100.0 |
|                           | $R^*$      | 1.1     | 2.8  | 5.3  | 95.3  | 97.7  | 99.1  |
|                           | $R^u$      | 0.8     | 2.1  | 4.1  | 95.2  | 97.6  | 99.0  |
|                           | $R^c$      | 1.1     | 2.7  | 5.1  | 95.4  | 97.6  | 99.0  |
|                           | $R_l^c$    | 1.2     | 3.0  | 5.8  | 94.9  | 97.4  | 98.8  |
|                           | $R_{ls}^c$ | 1.1     | 2.7  | 5.2  | 95.3  | 97.6  | 99.0  |
| Behrens-Fisher            | $R$        | 2.1     | 4.6  | 8.0  | 92.9  | 96.0  | 97.8  |
|                           | $R^*$      | 1.1     | 2.6  | 5.2  | 95.2  | 97.5  | 99.1  |
|                           | $R^u$      | 1.0     | 2.5  | 5.1  | 95.4  | 97.6  | 99.1  |
|                           | $R^c$      | 1.0     | 2.5  | 5.1  | 95.4  | 97.6  | 99.1  |
|                           | $R_l^c$    | 2.1     | 4.5  | 8.0  | 92.8  | 95.9  | 97.9  |
|                           | $R_{ls}^c$ | 1.0     | 2.5  | 5.2  | 95.4  | 97.5  | 99.1  |
| Logistic regression       | $R$        | 4.0     | 7.7  | 12.9 | 97.2  | 98.7  | 99.4  |
|                           | $R^*$      | 1.1     | 2.5  | 5.3  | 94.9  | 97.5  | 99.0  |
|                           | $R^u$      | 0.3     | 1.2  | 2.5  | 96.7  | 98.7  | 99.6  |
|                           | $R^c$      | 1.1     | 2.5  | 5.3  | 94.9  | 97.5  | 99.0  |
|                           | $R_l^c$    | 1.6     | 3.5  | 6.4  | 93.8  | 96.6  | 98.5  |
|                           | $R_{ls}^c$ | 1.1     | 2.6  | 5.3  | 94.9  | 97.5  | 99.0  |

Table S8: Empirical tail probabilities  $\times 100$  for the statistics in Table 1 of the main text and all models that have been considered in the simulation experiments. The figures shown have been rounded to 1 decimal and are for  $q = 100$  and  $m = 16$ .

| Model                     | Statistic  | Nominal |      |      |      |       |       |
|---------------------------|------------|---------|------|------|------|-------|-------|
|                           |            | 1.0     | 2.5  | 5.0  | 95.0 | 97.5  | 99.0  |
| Gamma                     | $R$        | 0.0     | 0.0  | 0.1  | 48.7 | 61.2  | 73.7  |
|                           | $R^*$      | 1.2     | 2.7  | 5.3  | 94.9 | 97.4  | 99.0  |
|                           | $R^u$      | 1.2     | 2.8  | 5.5  | 95.1 | 97.7  | 99.0  |
|                           | $R^c$      | 1.2     | 2.7  | 5.4  | 95.0 | 97.6  | 99.1  |
|                           | $R_l^c$    | 1.3     | 2.9  | 5.7  | 94.8 | 97.5  | 99.0  |
|                           | $R_{ls}^c$ | 1.3     | 2.8  | 5.5  | 95.1 | 97.6  | 99.1  |
| Beta                      | $R$        | 0.0     | 0.0  | 0.0  | 34.8 | 47.2  | 61.1  |
|                           | $R^*$      | 0.9     | 2.3  | 4.7  | 94.7 | 97.4  | 98.9  |
|                           | $R^u$      | 1.0     | 2.3  | 4.6  | 94.7 | 97.3  | 98.9  |
|                           | $R^c$      | 0.9     | 2.2  | 4.7  | 94.8 | 97.4  | 98.9  |
|                           | $R_l^c$    | 1.0     | 2.4  | 4.9  | 94.5 | 97.4  | 98.9  |
|                           | $R_{ls}^c$ | 1.0     | 2.4  | 4.8  | 94.8 | 97.4  | 98.9  |
| Curved exponential family | $R$        | 19.0    | 30.3 | 42.2 | 99.9 | 100.0 | 100.0 |
|                           | $R^*$      | 1.0     | 2.6  | 5.5  | 95.3 | 97.5  | 99.0  |
|                           | $R^u$      | 0.8     | 2.3  | 4.9  | 95.2 | 97.6  | 99.0  |
|                           | $R^c$      | 0.9     | 2.6  | 5.4  | 95.2 | 97.5  | 99.0  |
|                           | $R_l^c$    | 1.1     | 2.8  | 5.6  | 95.0 | 97.4  | 98.9  |
|                           | $R_{ls}^c$ | 1.0     | 2.6  | 5.4  | 95.2 | 97.5  | 99.0  |
| Behrens-Fisher            | $R$        | 1.7     | 3.6  | 6.6  | 93.4 | 96.4  | 98.4  |
|                           | $R^*$      | 1.2     | 2.8  | 5.4  | 94.6 | 97.4  | 98.9  |
|                           | $R^u$      | 1.1     | 2.8  | 5.3  | 94.6 | 97.4  | 98.9  |
|                           | $R^c$      | 1.1     | 2.7  | 5.3  | 94.6 | 97.4  | 98.9  |
|                           | $R_l^c$    | 1.7     | 3.6  | 6.7  | 93.3 | 96.4  | 98.4  |
|                           | $R_{ls}^c$ | 1.1     | 2.9  | 5.4  | 94.5 | 97.4  | 98.9  |
| Logistic regression       | $R$        | 2.7     | 5.9  | 10.0 | 97.0 | 98.6  | 99.4  |
|                           | $R^*$      | 1.1     | 2.8  | 5.5  | 95.0 | 97.6  | 99.1  |
|                           | $R^u$      | 0.7     | 1.9  | 4.2  | 96.0 | 98.2  | 99.3  |
|                           | $R^c$      | 1.1     | 2.8  | 5.6  | 95.1 | 97.6  | 99.0  |
|                           | $R_l^c$    | 1.4     | 3.2  | 6.2  | 94.5 | 97.2  | 98.9  |
|                           | $R_{ls}^c$ | 1.1     | 2.8  | 5.5  | 95.0 | 97.6  | 99.1  |

Table S9: Empirical tail probabilities  $\times 100$  for the statistics in Table 1 of the main text and all models that have been considered in the simulation experiments. The figures shown have been rounded to 1 decimal and are for  $q = 1000$  and  $m = 4$ .

| Model                     | Statistic  | Nominal |       |       |       |       |       |
|---------------------------|------------|---------|-------|-------|-------|-------|-------|
|                           |            | 1.0     | 2.5   | 5.0   | 95.0  | 97.5  | 99.0  |
| Gamma                     | $R$        | 0.0     | 0.0   | 0.0   | 0.0   | 0.0   | 0.0   |
|                           | $R^*$      | 0.2     | 0.5   | 1.2   | 83.7  | 90.3  | 95.3  |
|                           | $R^u$      | 1.3     | 3.2   | 6.4   | 96.4  | 98.2  | 99.2  |
|                           | $R^c$      | 1.0     | 2.5   | 5.1   | 94.8  | 97.4  | 98.9  |
|                           | $R_l^c$    | 1.4     | 3.1   | 6.2   | 93.9  | 96.7  | 98.5  |
|                           | $R_{ls}^c$ | 1.0     | 2.5   | 5.1   | 95.0  | 97.4  | 98.9  |
| Beta                      | $R$        | 0.0     | 0.0   | 0.0   | 0.0   | 0.0   | 0.0   |
|                           | $R^*$      | 0.3     | 0.8   | 1.8   | 88.6  | 93.5  | 96.7  |
|                           | $R^u$      | 0.5     | 1.3   | 2.8   | 91.4  | 94.9  | 97.6  |
|                           | $R^c$      | 0.7     | 1.9   | 3.8   | 93.7  | 96.4  | 98.6  |
|                           | $R_l^c$    | 1.0     | 2.3   | 4.6   | 92.9  | 95.7  | 98.1  |
|                           | $R_{ls}^c$ | 0.8     | 1.8   | 3.9   | 93.7  | 96.5  | 98.5  |
| Curved exponential family | $R$        | 100.0   | 100.0 | 100.0 | 100.0 | 100.0 | 100.0 |
|                           | $R^*$      | 3.2     | 6.3   | 10.6  | 97.8  | 99.0  | 99.6  |
|                           | $R^u$      | 0.4     | 1.3   | 2.7   | 92.8  | 96.4  | 98.5  |
|                           | $R^c$      | 2.2     | 4.8   | 8.3   | 96.9  | 98.5  | 99.4  |
|                           | $R_l^c$    | 3.1     | 6.0   | 9.8   | 96.2  | 98.0  | 99.2  |
|                           | $R_{ls}^c$ | 2.4     | 4.9   | 8.3   | 96.9  | 98.6  | 99.4  |
| Behrens-Fisher            | $R$        | 5.3     | 8.7   | 12.3  | 87.8  | 92.0  | 95.1  |
|                           | $R^*$      | 1.5     | 3.3   | 6.3   | 94.1  | 96.8  | 98.6  |
|                           | $R^u$      | 1.0     | 2.6   | 5.2   | 95.1  | 97.5  | 99.0  |
|                           | $R^c$      | 1.0     | 2.7   | 5.1   | 95.1  | 97.5  | 99.1  |
|                           | $R_l^c$    | 5.3     | 8.7   | 12.3  | 87.8  | 92.0  | 95.1  |
|                           | $R_{ls}^c$ | 1.1     | 2.7   | 5.1   | 95.1  | 97.4  | 99.0  |
| Logistic regression       | $R$        | 40.2    | 53.2  | 64.3  | 99.9  | 100.0 | 100.0 |
|                           | $R^*$      | 2.0     | 4.5   | 8.3   | 97.1  | 98.5  | 99.5  |
|                           | $R^u$      | 0.0     | 0.1   | 0.5   | 97.2  | 98.9  | 99.8  |
|                           | $R^c$      | 1.8     | 4.2   | 8.1   | 97.0  | 98.5  | 99.4  |
|                           | $R_l^c$    | 3.7     | 7.5   | 11.8  | 95.2  | 97.3  | 98.7  |
|                           | $R_{ls}^c$ | 1.8     | 4.2   | 8.2   | 97.0  | 98.5  | 99.5  |

Table S10: Empirical tail probabilities  $\times 100$  for the statistics in Table 1 of the main text and all models that have been considered in the simulation experiments. The figures shown have been rounded to 1 decimal and are for  $q = 1000$  and  $m = 8$ . The first 4 blocks of rows are identical to Table 2 of the main text.

| Model                     | Statistic  | Nominal |       |       |       |       |       |
|---------------------------|------------|---------|-------|-------|-------|-------|-------|
|                           |            | 1.0     | 2.5   | 5.0   | 95.0  | 97.5  | 99.0  |
| Gamma                     | $R$        | 0.0     | 0.0   | 0.0   | 0.0   | 0.0   | 0.0   |
|                           | $R^*$      | 0.7     | 1.5   | 3.3   | 92.1  | 95.5  | 98.2  |
|                           | $R^u$      | 1.1     | 2.7   | 5.3   | 95.1  | 97.7  | 99.2  |
|                           | $R^c$      | 1.0     | 2.5   | 5.0   | 94.6  | 97.2  | 99.0  |
|                           | $R_l^c$    | 1.1     | 2.8   | 5.4   | 94.2  | 96.8  | 98.9  |
|                           | $R_{ls}^c$ | 1.1     | 2.5   | 4.9   | 94.5  | 97.2  | 99.1  |
| Beta                      | $R$        | 0.0     | 0.0   | 0.0   | 0.0   | 0.0   | 0.0   |
|                           | $R^*$      | 0.7     | 1.8   | 3.8   | 93.7  | 96.8  | 98.8  |
|                           | $R^u$      | 0.8     | 1.9   | 4.1   | 94.0  | 97.0  | 98.7  |
|                           | $R^c$      | 1.0     | 2.3   | 4.8   | 95.0  | 97.4  | 99.1  |
|                           | $R_l^c$    | 1.1     | 2.5   | 5.1   | 94.7  | 97.3  | 98.9  |
|                           | $R_{ls}^c$ | 0.9     | 2.3   | 4.8   | 95.1  | 97.5  | 99.0  |
| Curved exponential family | $R$        | 100.0   | 100.0 | 100.0 | 100.0 | 100.0 | 100.0 |
|                           | $R^*$      | 1.4     | 3.5   | 6.9   | 96.6  | 98.3  | 99.4  |
|                           | $R^u$      | 0.6     | 1.8   | 4.0   | 95.0  | 97.7  | 99.2  |
|                           | $R^c$      | 1.2     | 3.3   | 6.4   | 96.2  | 98.2  | 99.4  |
|                           | $R_l^c$    | 1.5     | 3.6   | 7.1   | 95.8  | 98.0  | 99.2  |
|                           | $R_{ls}^c$ | 1.3     | 3.2   | 6.5   | 96.3  | 98.2  | 99.4  |
| Behrens-Fisher            | $R$        | 2.4     | 4.6   | 7.6   | 92.1  | 95.6  | 98.0  |
|                           | $R^*$      | 1.2     | 2.8   | 5.3   | 94.8  | 97.5  | 99.0  |
|                           | $R^u$      | 1.1     | 2.7   | 5.2   | 95.0  | 97.6  | 99.1  |
|                           | $R^c$      | 1.1     | 2.7   | 5.1   | 94.9  | 97.6  | 99.1  |
|                           | $R_l^c$    | 2.4     | 4.7   | 7.6   | 92.1  | 95.5  | 98.0  |
|                           | $R_{ls}^c$ | 1.1     | 2.6   | 5.1   | 95.0  | 97.6  | 99.1  |
| Logistic regression       | $R$        | 18.1    | 28.4  | 39.3  | 99.7  | 99.9  | 100.0 |
|                           | $R^*$      | 1.4     | 3.1   | 6.1   | 95.8  | 97.9  | 99.1  |
|                           | $R^u$      | 0.4     | 1.1   | 2.4   | 96.3  | 98.4  | 99.4  |
|                           | $R^c$      | 1.5     | 3.1   | 6.0   | 95.8  | 97.9  | 99.2  |
|                           | $R_l^c$    | 1.9     | 4.1   | 7.5   | 94.7  | 97.1  | 98.8  |
|                           | $R_{ls}^c$ | 1.4     | 3.2   | 6.0   | 95.8  | 97.9  | 99.1  |

Table S11: Empirical tail probabilities  $\times 100$  for the statistics in Table 1 of the main text and all models that have been considered in the simulation experiments. The figures shown have been rounded to 1 decimal and are for  $q = 1000$  and  $m = 16$ .

| Model                     | Statistic  | Nominal |      |      |       |       |       |
|---------------------------|------------|---------|------|------|-------|-------|-------|
|                           |            | 1.0     | 2.5  | 5.0  | 95.0  | 97.5  | 99.0  |
| Gamma                     | $R$        | 0.0     | 0.0  | 0.0  | 0.0   | 0.0   | 0.2   |
|                           | $R^*$      | 0.9     | 2.1  | 4.3  | 94.3  | 96.9  | 98.5  |
|                           | $R^u$      | 1.1     | 2.5  | 5.0  | 95.2  | 97.6  | 98.9  |
|                           | $R^c$      | 1.0     | 2.5  | 4.9  | 95.0  | 97.5  | 98.9  |
|                           | $R_l^c$    | 1.1     | 2.6  | 5.1  | 94.8  | 97.3  | 98.6  |
|                           | $R_{ls}^c$ | 1.1     | 2.5  | 5.0  | 95.0  | 97.5  | 98.8  |
| Beta                      | $R$        | 0.0     | 0.0  | 0.0  | 0.0   | 0.0   | 0.0   |
|                           | $R^*$      | 1.0     | 2.3  | 4.5  | 94.3  | 97.2  | 98.8  |
|                           | $R^u$      | 1.1     | 2.3  | 4.7  | 94.4  | 97.2  | 98.8  |
|                           | $R^c$      | 1.0     | 2.4  | 4.8  | 94.8  | 97.4  | 99.0  |
|                           | $R_l^c$    | 1.2     | 2.5  | 5.0  | 94.7  | 97.3  | 98.9  |
|                           | $R_{ls}^c$ | 1.1     | 2.4  | 4.9  | 94.8  | 97.4  | 98.9  |
| Curved exponential family | $R$        | 98.2    | 99.3 | 99.7 | 100.0 | 100.0 | 100.0 |
|                           | $R^*$      | 1.0     | 2.8  | 5.5  | 95.9  | 98.1  | 99.3  |
|                           | $R^u$      | 0.7     | 2.1  | 4.5  | 95.3  | 97.9  | 99.3  |
|                           | $R^c$      | 1.1     | 2.6  | 5.4  | 95.7  | 98.1  | 99.3  |
|                           | $R_l^c$    | 1.1     | 2.8  | 5.7  | 95.5  | 97.9  | 99.2  |
|                           | $R_{ls}^c$ | 1.0     | 2.6  | 5.4  | 95.7  | 98.0  | 99.3  |
| Behrens-Fisher            | $R$        | 1.5     | 3.4  | 6.1  | 93.9  | 96.6  | 98.5  |
|                           | $R^*$      | 1.1     | 2.6  | 5.0  | 94.9  | 97.5  | 98.9  |
|                           | $R^u$      | 1.1     | 2.6  | 5.0  | 95.0  | 97.5  | 99.1  |
|                           | $R^c$      | 1.1     | 2.6  | 5.0  | 95.1  | 97.5  | 99.1  |
|                           | $R_l^c$    | 1.5     | 3.4  | 6.2  | 93.8  | 96.7  | 98.5  |
|                           | $R_{ls}^c$ | 1.1     | 2.6  | 4.9  | 95.0  | 97.5  | 99.0  |
| Logistic regression       | $R$        | 8.5     | 15.2 | 23.7 | 99.3  | 99.7  | 100.0 |
|                           | $R^*$      | 1.3     | 2.9  | 5.5  | 95.1  | 97.7  | 99.0  |
|                           | $R^u$      | 0.7     | 1.9  | 3.9  | 95.5  | 98.0  | 99.2  |
|                           | $R^c$      | 1.3     | 2.9  | 5.5  | 95.1  | 97.6  | 99.0  |
|                           | $R_l^c$    | 1.6     | 3.4  | 6.0  | 94.7  | 97.2  | 98.9  |
|                           | $R_{ls}^c$ | 1.3     | 2.9  | 5.5  | 95.1  | 97.6  | 99.1  |
